# Supplementary material for: Predicting the Price Movement of Cryptocurrencies Using Linear Law-based Transformation
Source: arXiv:2305.04884 source file (2023-04-27)
Supplement: Supplementary file 1 [file supplementary_material.pdf]

# Supplementary Material for Predicting the Price Movement of Cryptocurrencies Using Linear Law-based Transformation

Marcell T. Kurbucz[a,b,*], Péter Pósfay[a], Antal Jakovác[a]

[a]*Department of Computational Sciences, Wigner Research Centre for Physics, 29-33 Konkoly-Thege Miklós Street, H-1121 Budapest, Hungary*
[b]*Institute of Data Analytics and Information Systems, Corvinus University of Budapest, 8 Fővám Square, H-1093, Hungary*

## Abstract

The aim of this paper is to investigate the effect of a novel method called linear law-based feature space transformation (LLT) on the accuracy of intraday price movement prediction of cryptocurrencies. To do this, the 1-minute interval price data of Bitcoin, Ethereum, Binance Coin, and Ripple between 1 January 2019 and 22 October 2022 were collected from the Binance cryptocurrency exchange. Then, 14-hour nonoverlapping time windows were applied to sample the price data. The classification was based on the first 12 hours, and the two classes were determined based on whether the closing price rose or fell after the next 2 hours. These price data were first transformed with the LLT, then they were classified by traditional machine learning algorithms with 10-fold cross-validation. Based on the results, LLT greatly increased the accuracy for all cryptocurrencies, which emphasizes the potential of the LLT algorithm in predicting price movements.

*Keywords:* Time series classification, Linear law, Feature space transformation, Feature engineering, Cryptocurrency, Artificial intelligence

## Contents

Optimization results . . . . . . . . . . . . . . . . . . . . 2
Confusion matrices . . . . . . . . . . . . . . . . . . . . 18

*Corresponding author: Tel.: +36 1 392 2222;
*Email addresses:* `kurbucz.marcell@wigner.hu` (Marcell T. Kurbucz), `posfay.peter@wigner.hu` (Péter Pósfay), `jakovac.antal@wigner.hu` (Antal Jakovác)

Figure S1: Optimization results

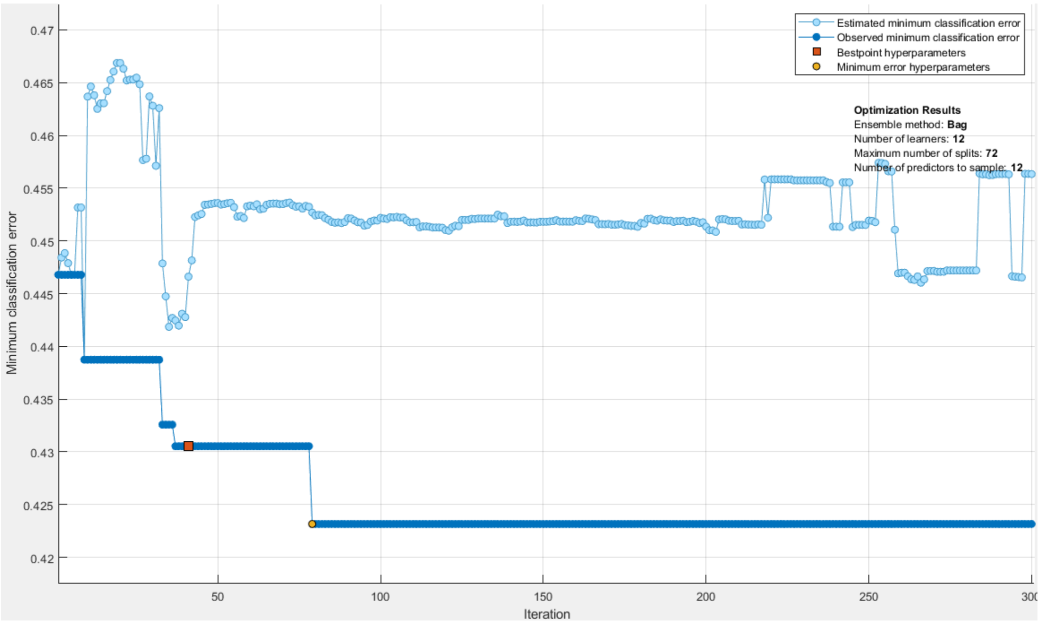


(a) Ensemble, BTC, original fs.

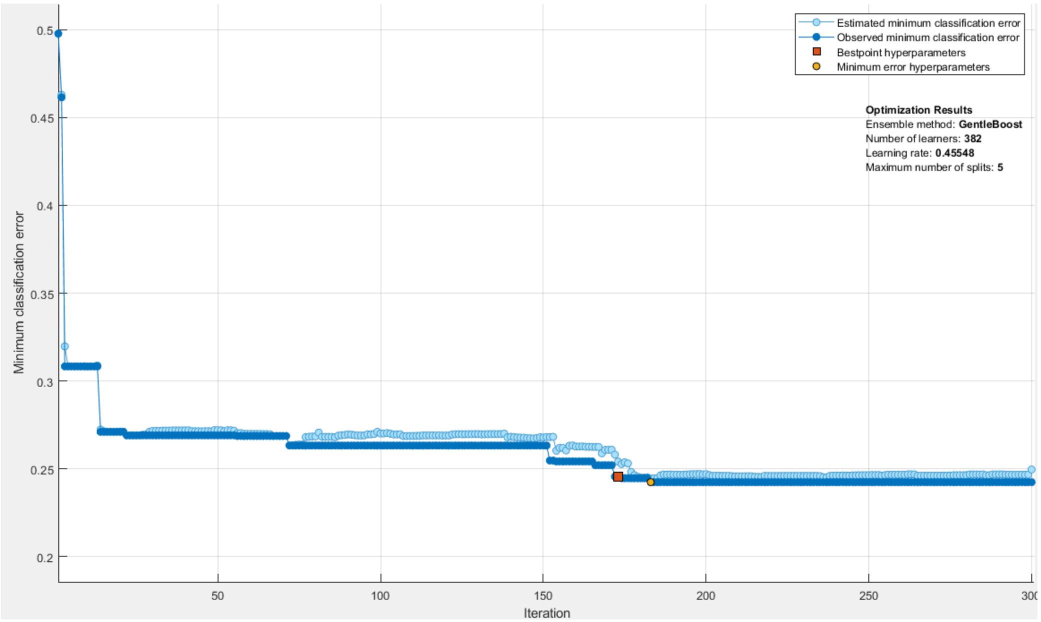


(b) Ensemble, BTC, LLT-based fs.

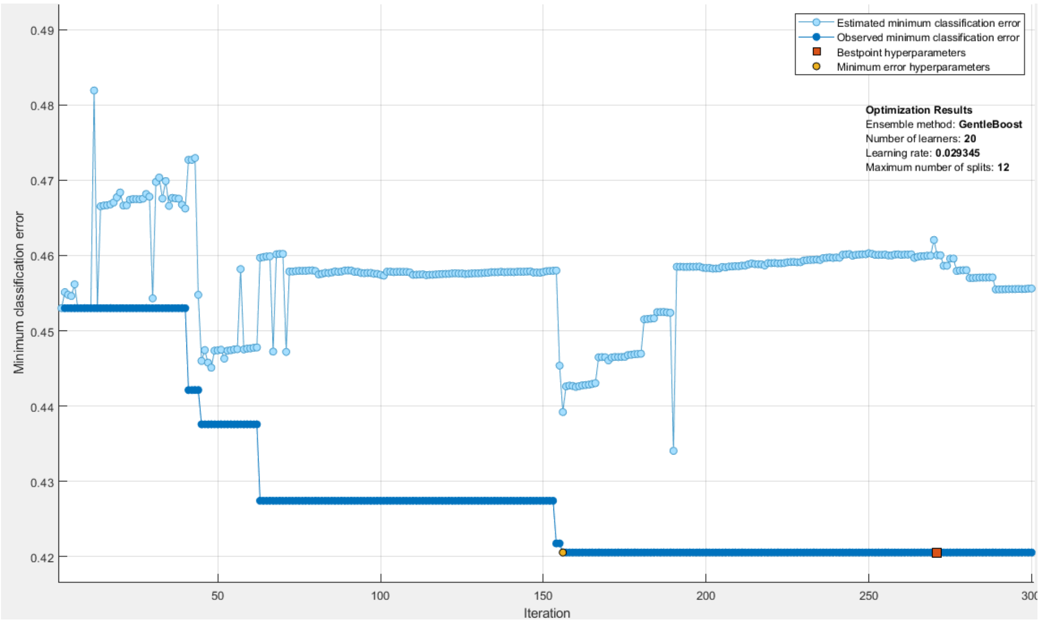


(c) Ensemble, ETH, original fs.

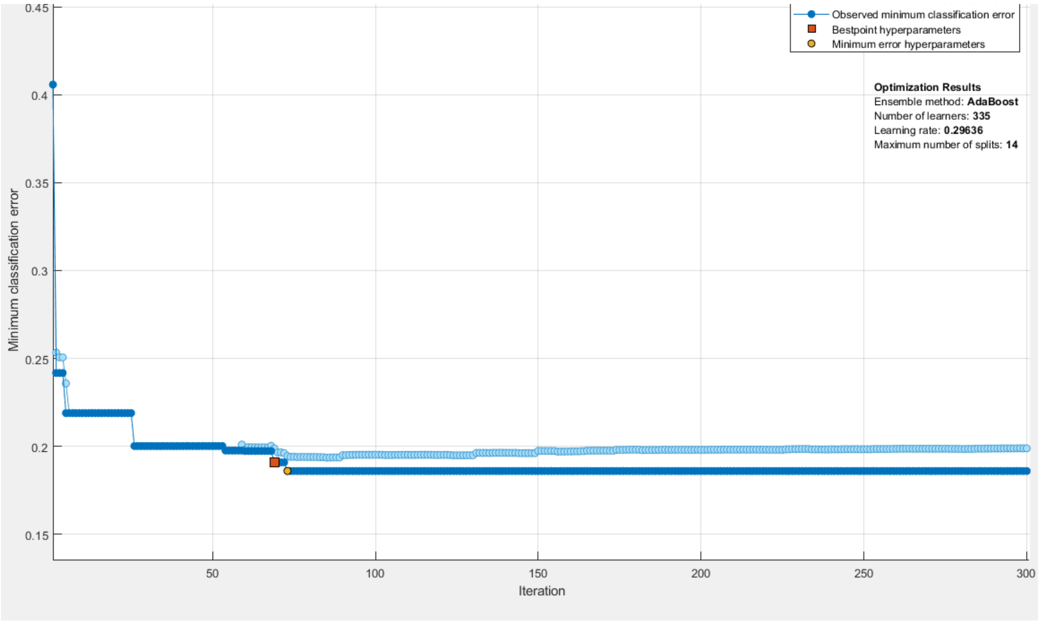


(d) Ensemble, ETH, LLT-based fs.

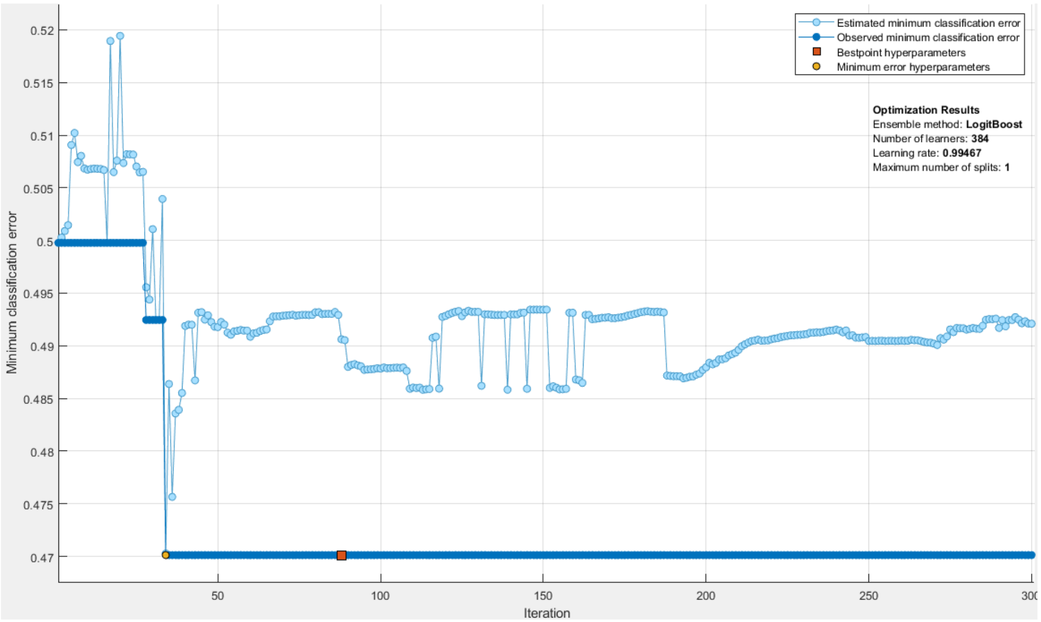


(e) Ensemble, BNB, original fs.

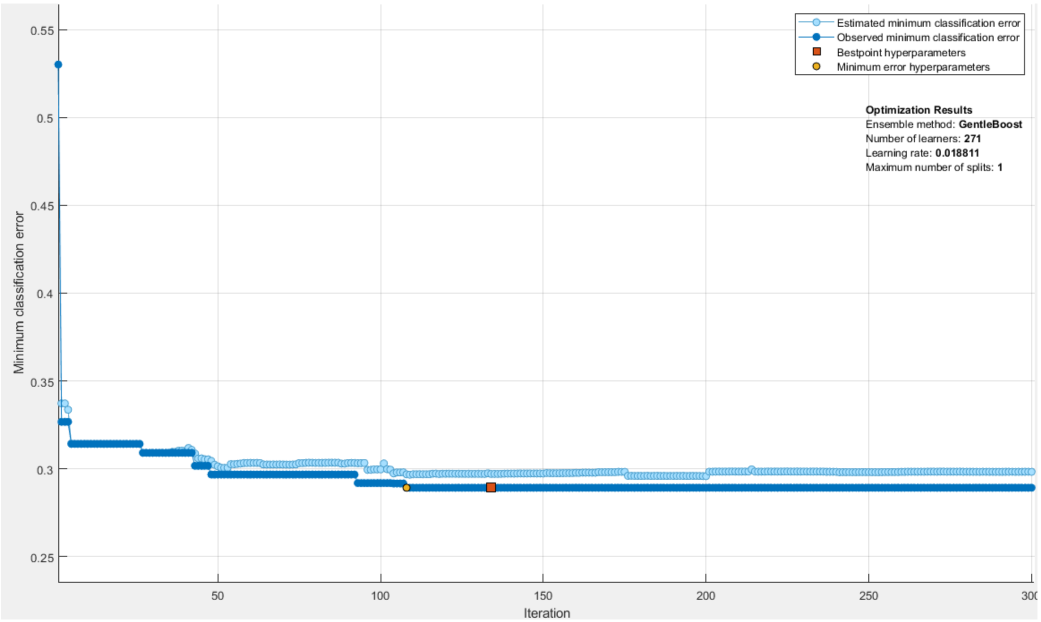


(f) Ensemble, BNB, LLT-based fs.

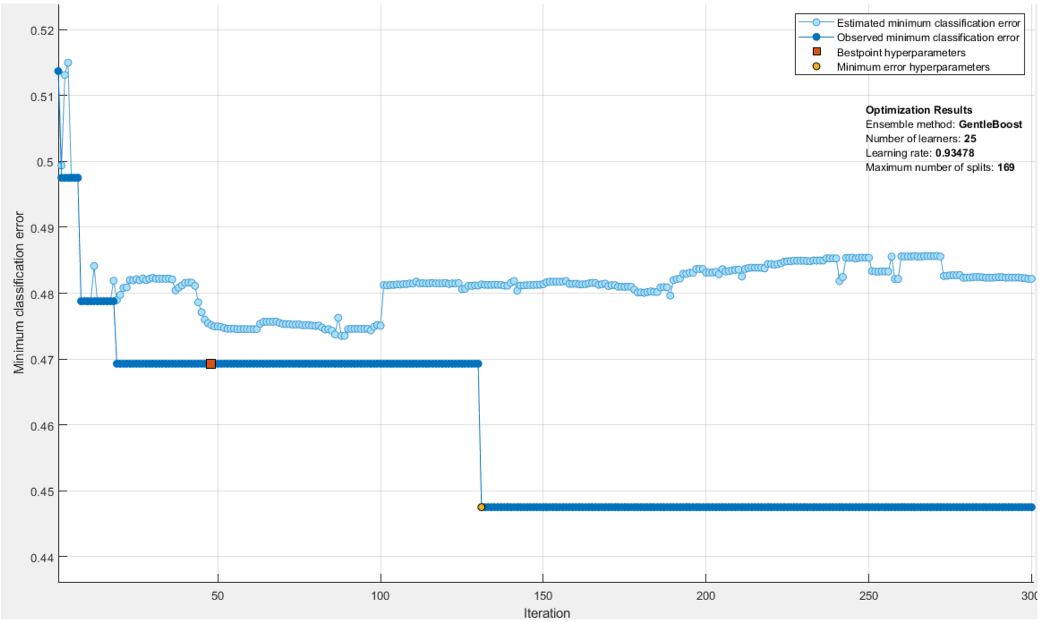


(g) Ensemble, XRB, original fs.

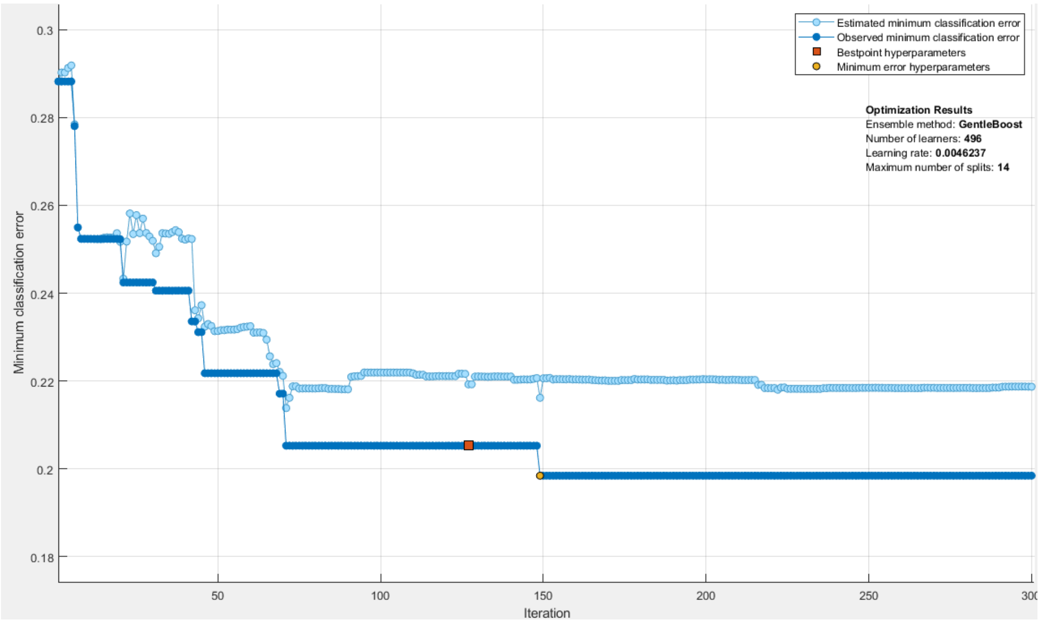


(h) Ensemble, XRB, LLT-based fs.

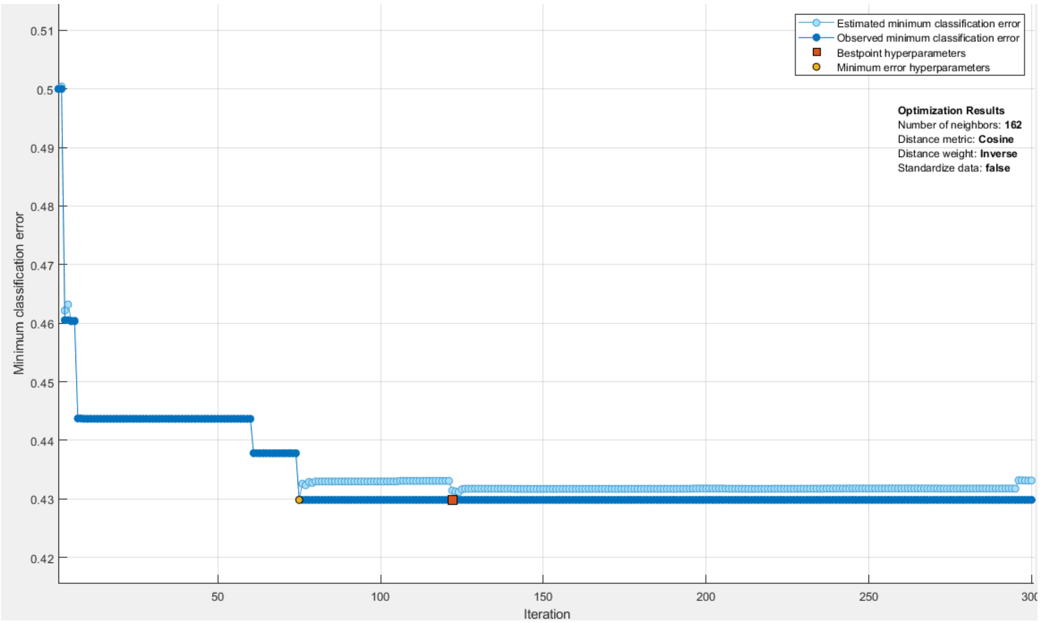


(i) KNN, BTC, original fs.

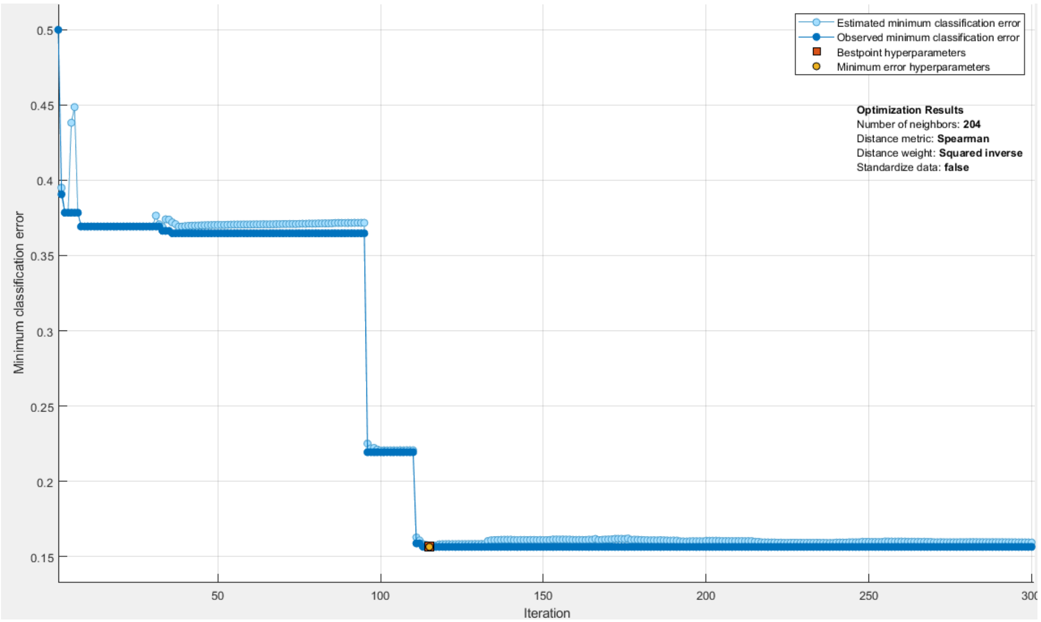


(j) KNN, BTC, LLT-based fs.

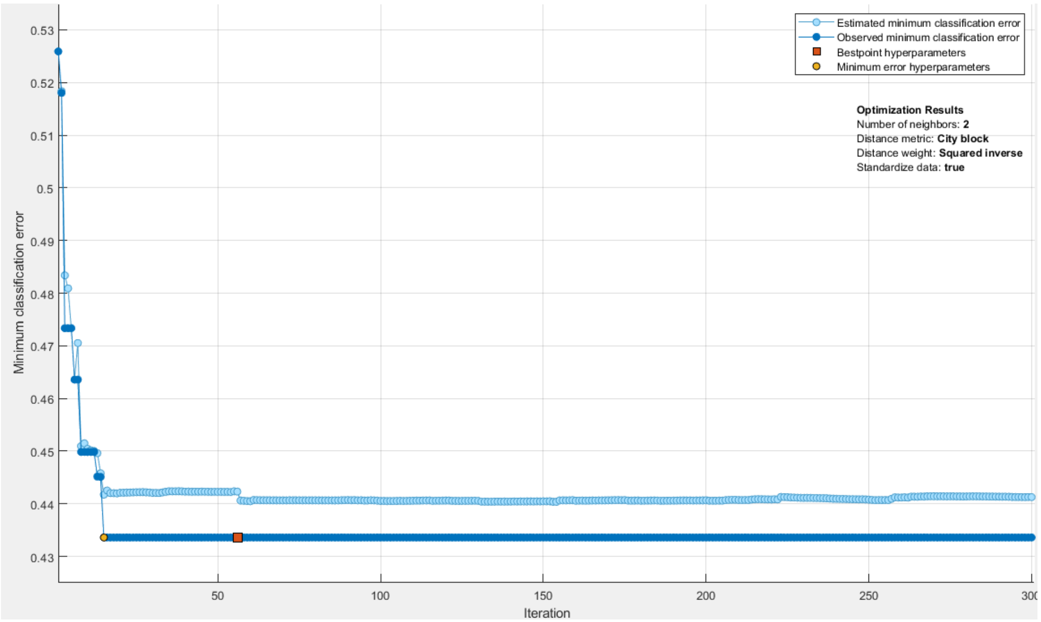


(k) KNN, ETH, original fs.

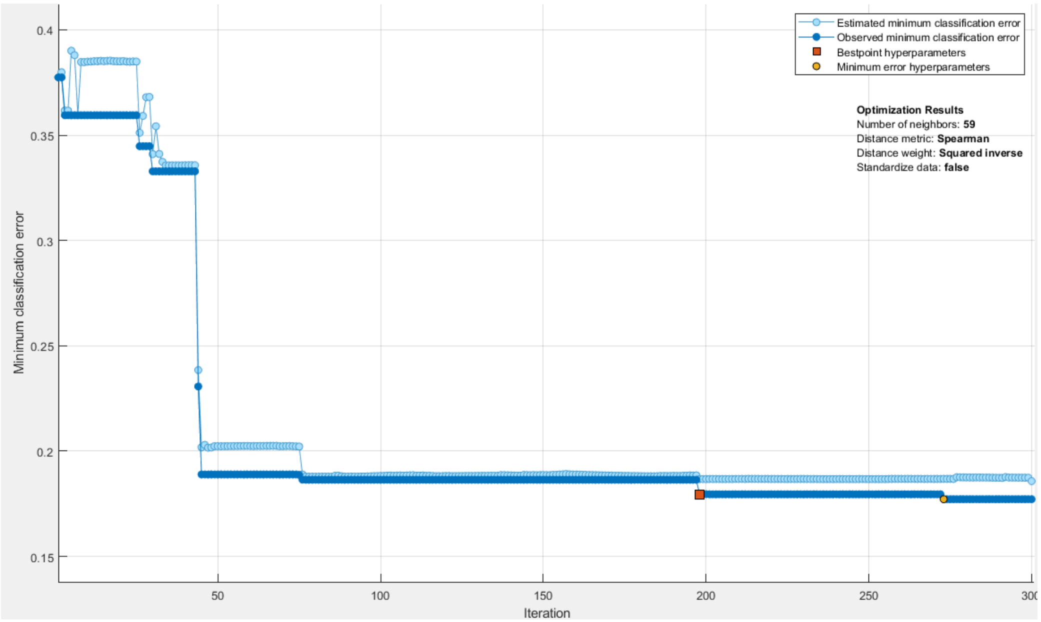


(l) KNN, ETH, LLT-based fs.

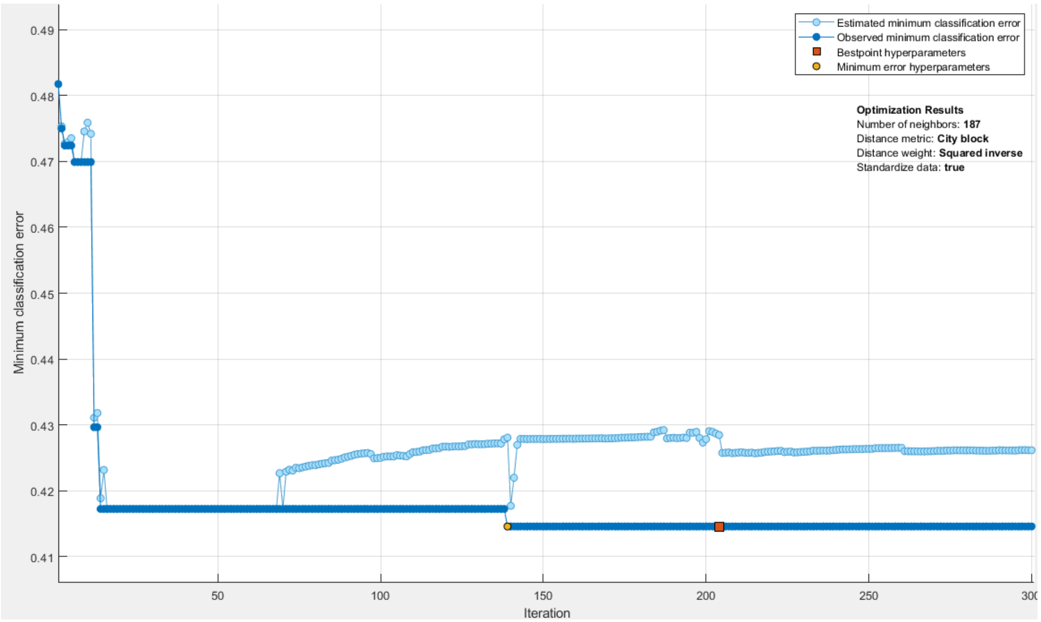


(m) KNN, BNB, original fs.

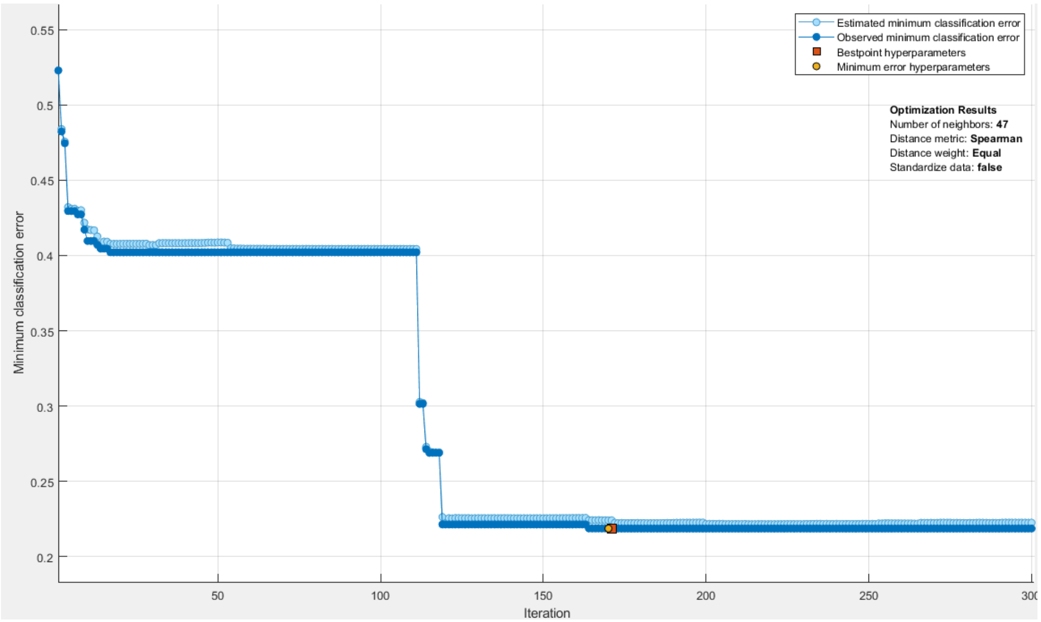


(n) KNN, BNB, LLT-based fs.

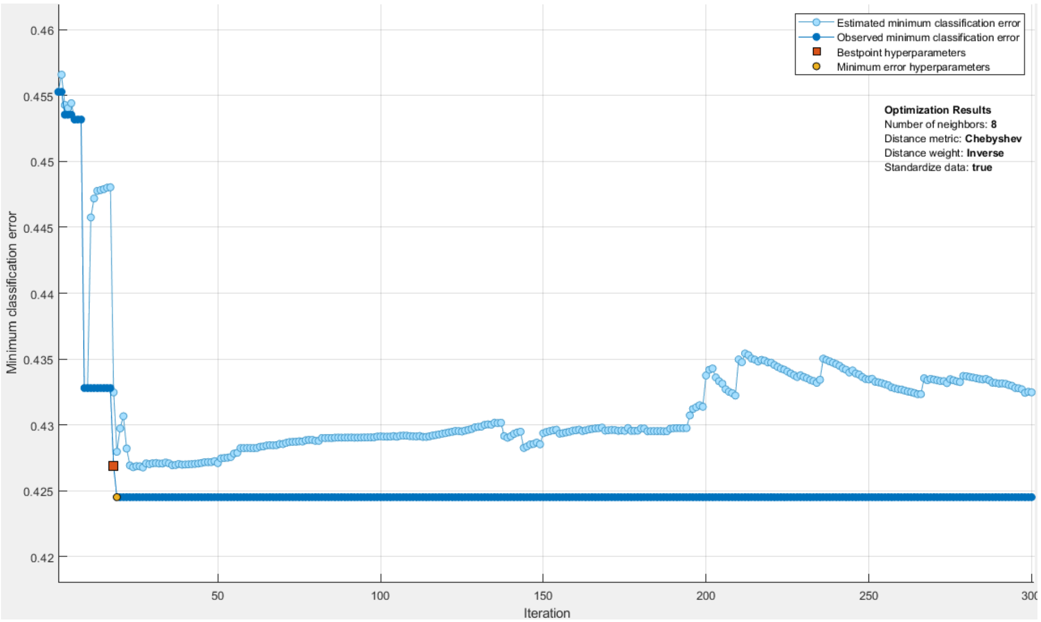


(o) KNN, XRB, original fs.

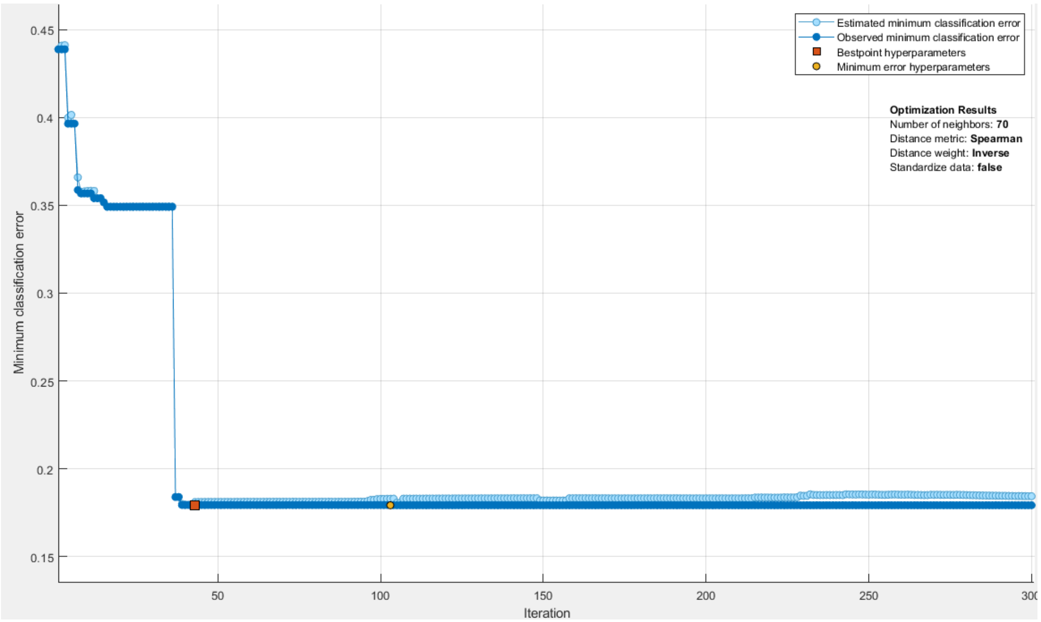


(p) KNN, XRB, LLT-based fs.

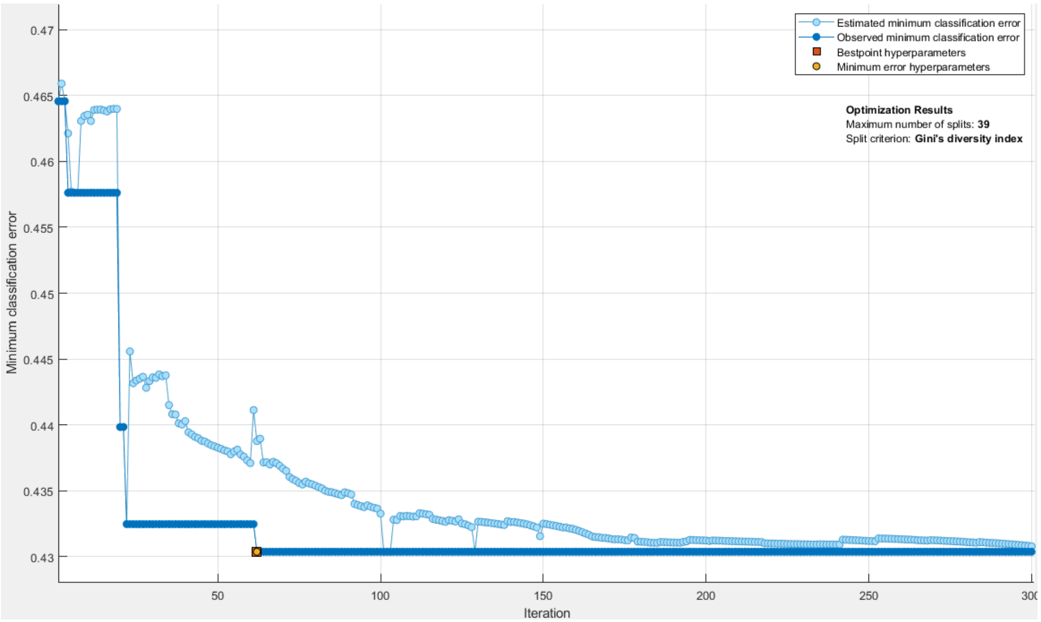


(q) DT, BTC, original fs.

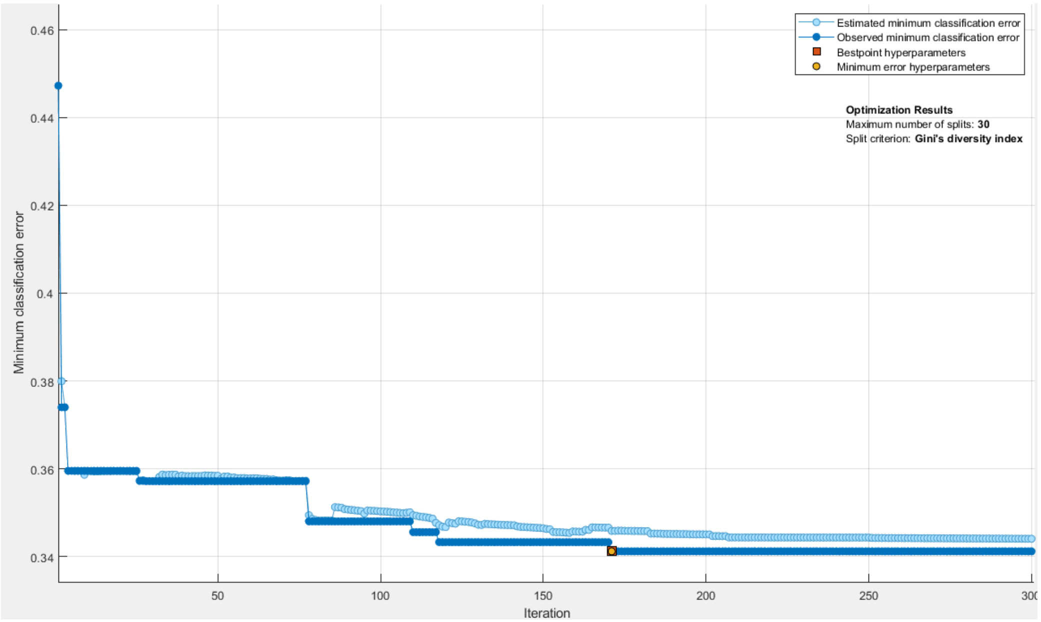


(r) DT, BTC, LLT-based fs.

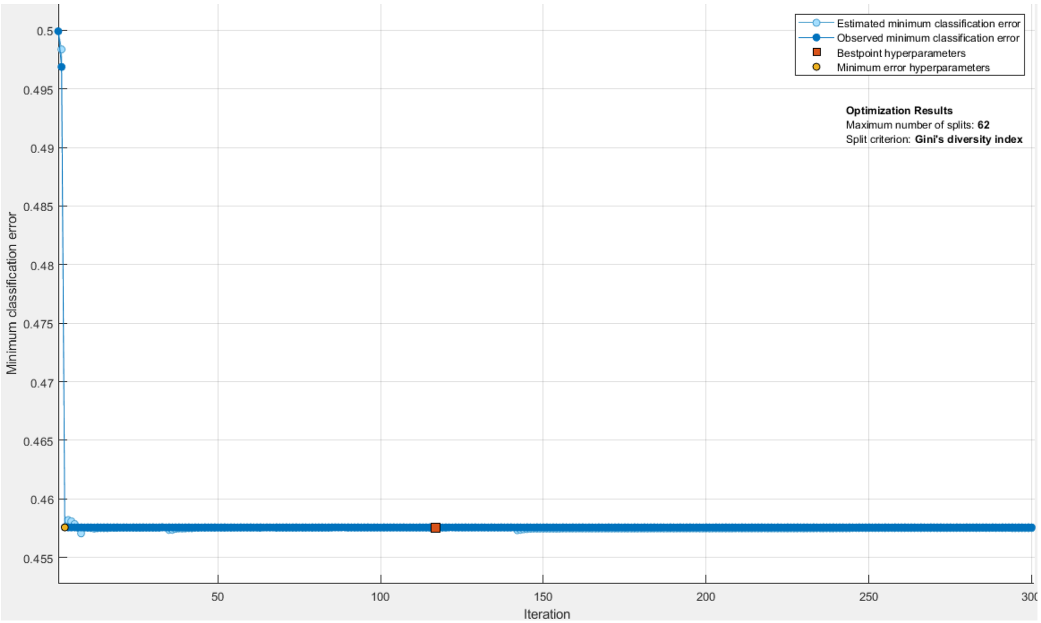


(s) DT, ETH, original fs.

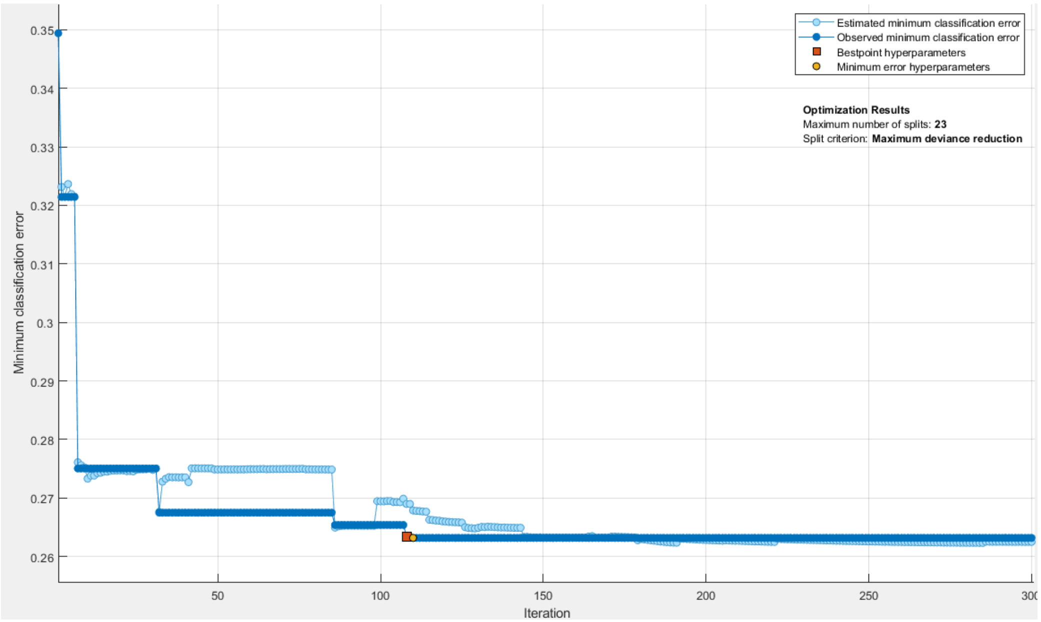


(t) DT, ETH, LLT-based fs.

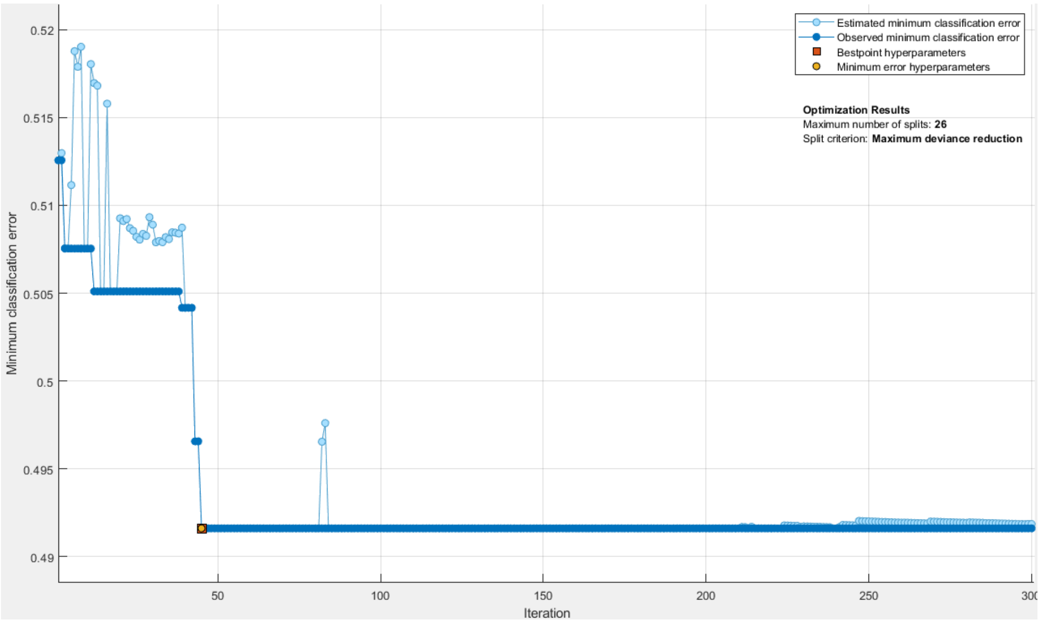


(u) DT, BNB, original fs.

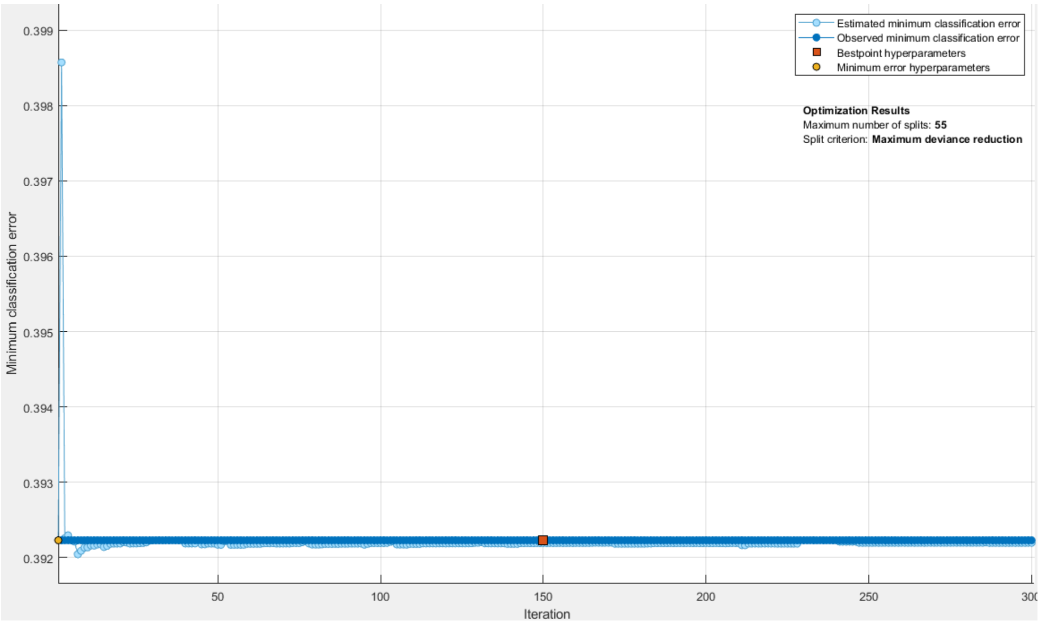


(v) DT, BNB, LLT-based fs.

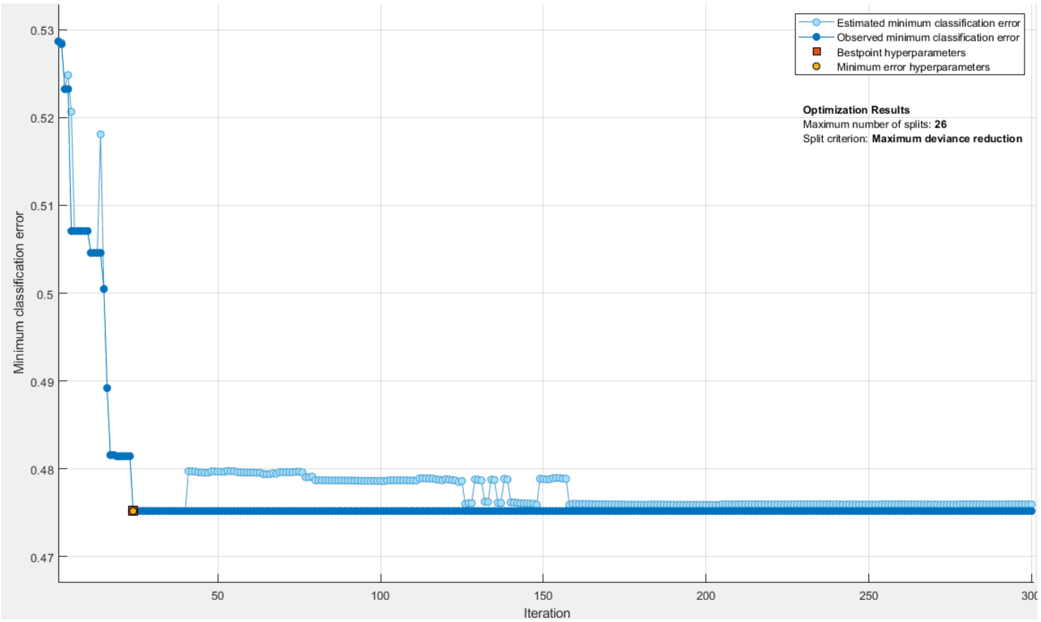


(w) DT, XRB, original fs.

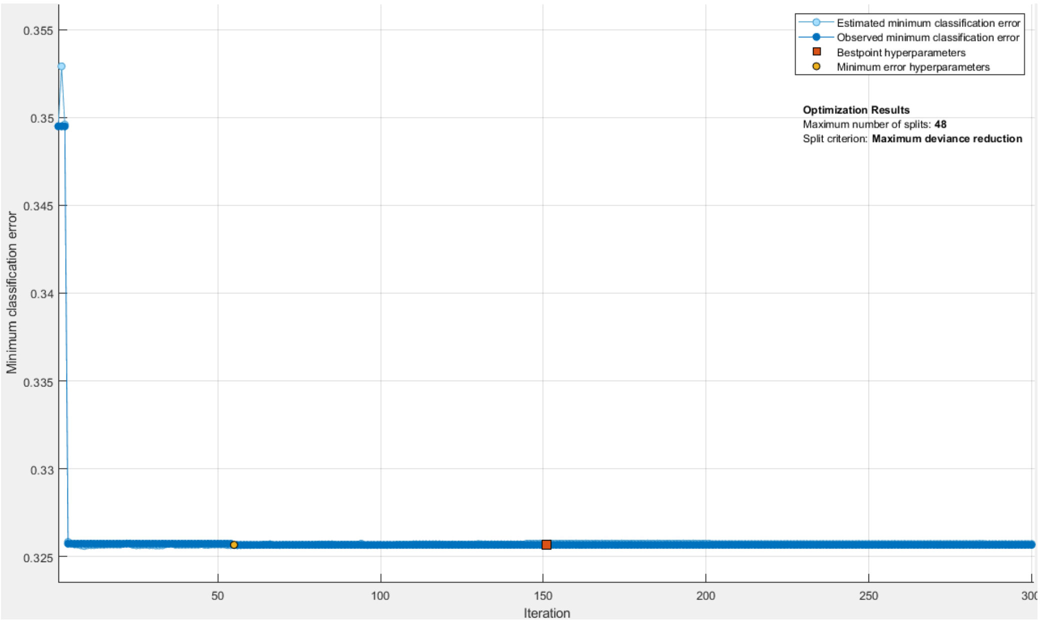


(x) DT, XRB, LLT-based fs.

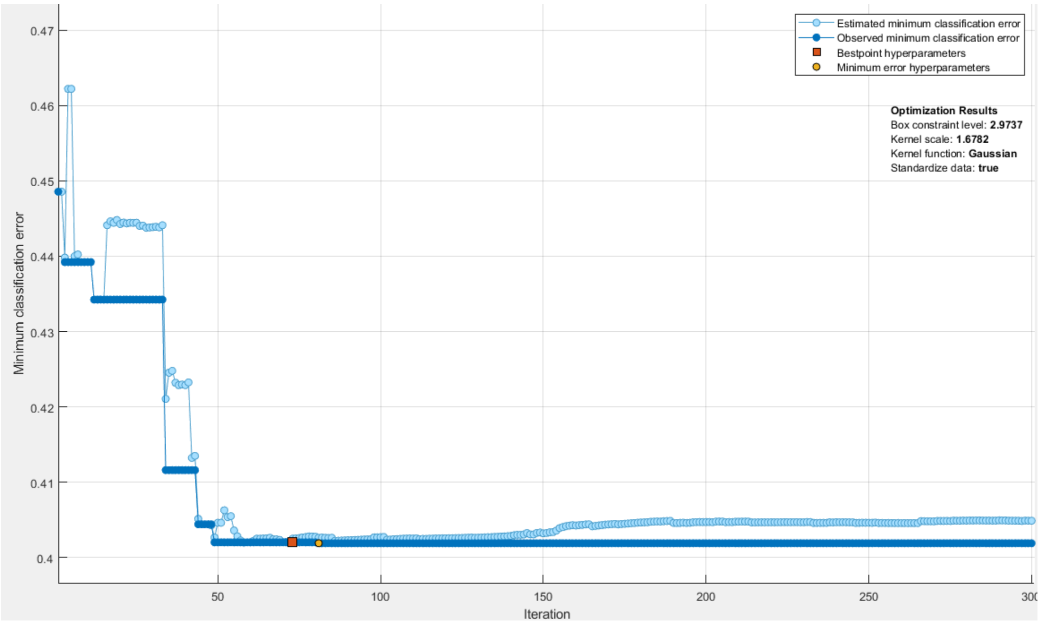


(y) SVM, BTC, original fs.

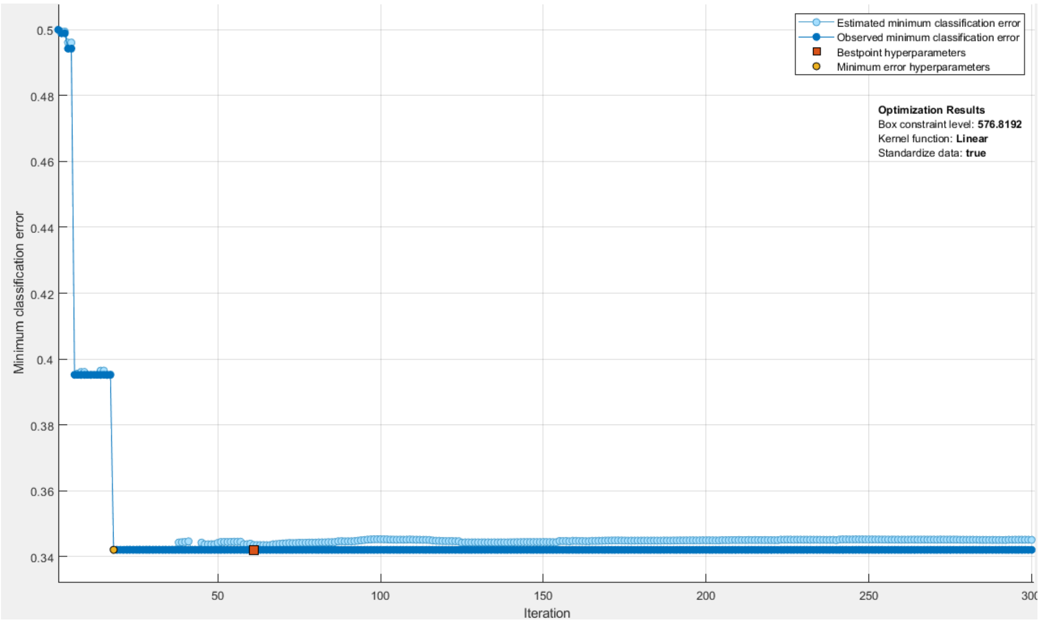


(z) SVM, BTC, LLT-based fs.

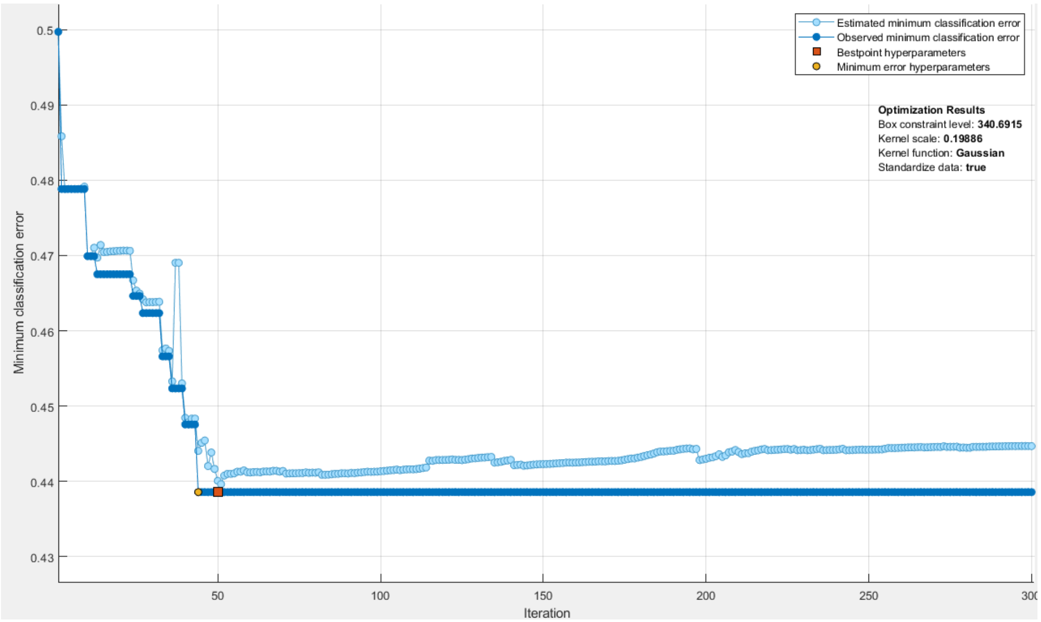


(aa) SVM, ETH, original fs.

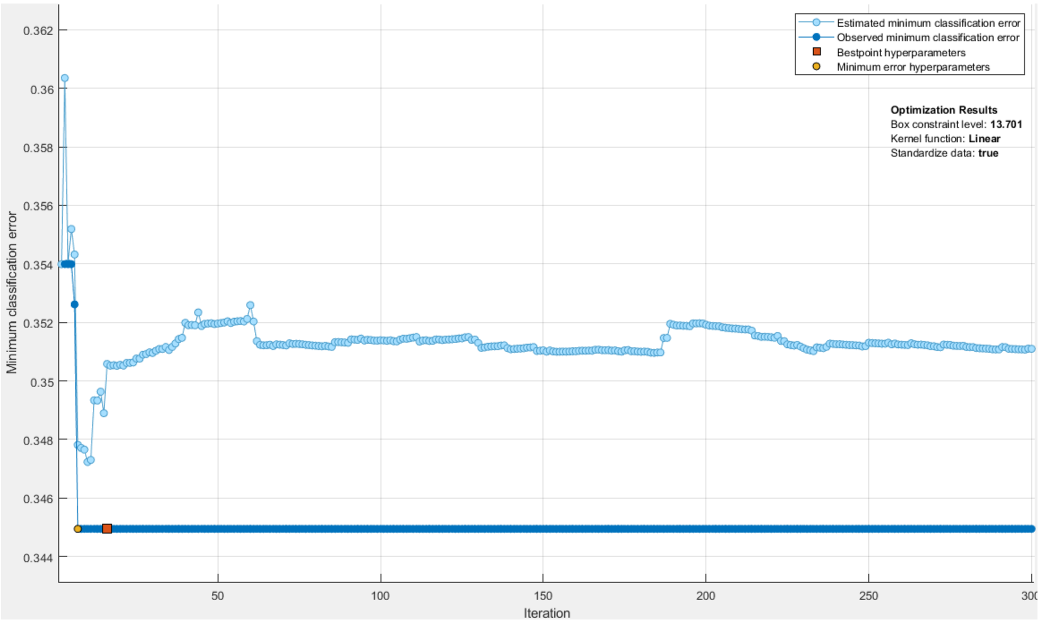


(ab) SVM, ETH, LLT-based fs.

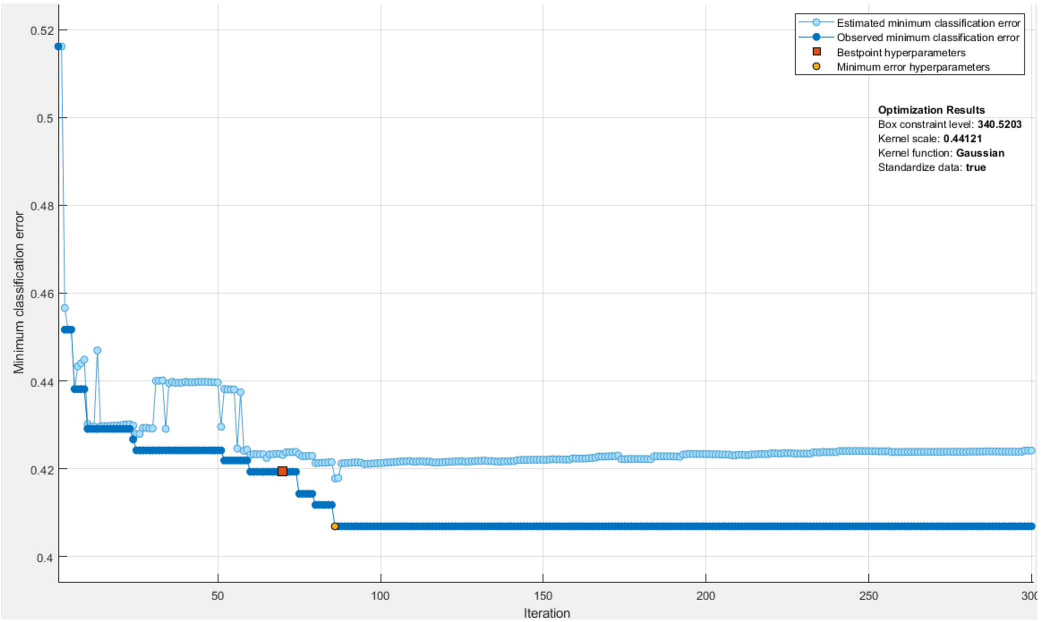


(ac) SVM, BNB, original fs.

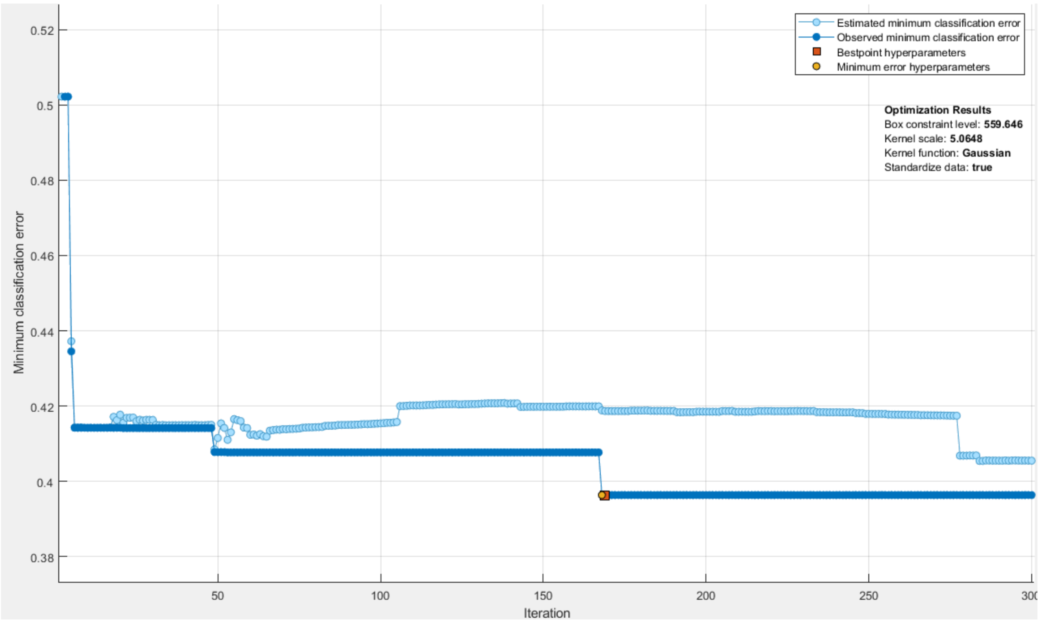


(ad) SVM, BNB, LLT-based fs.

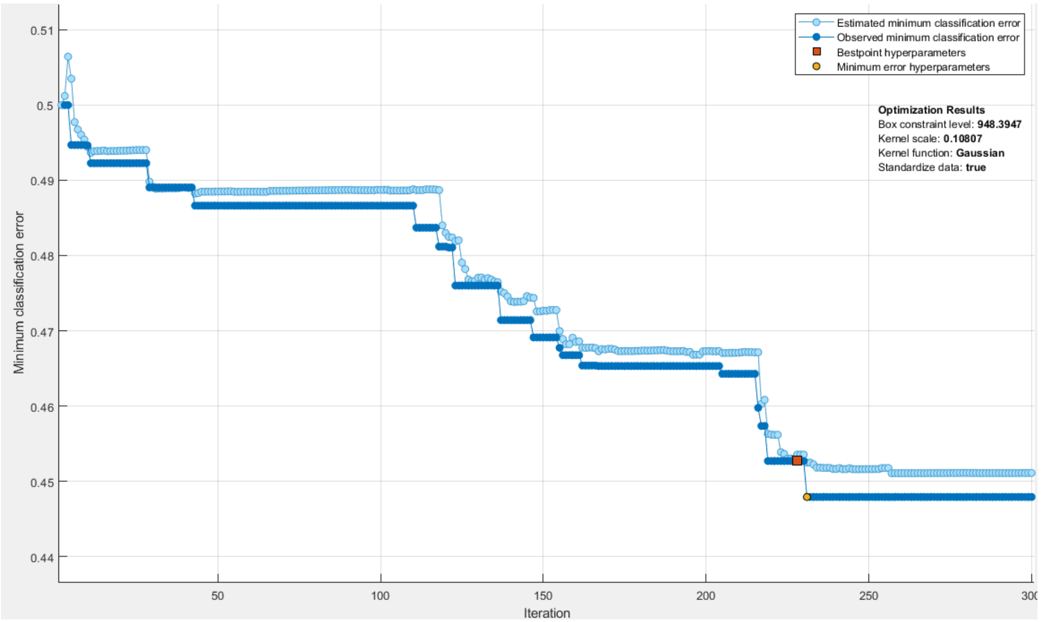


(ae) SVM, XRB, original fs.

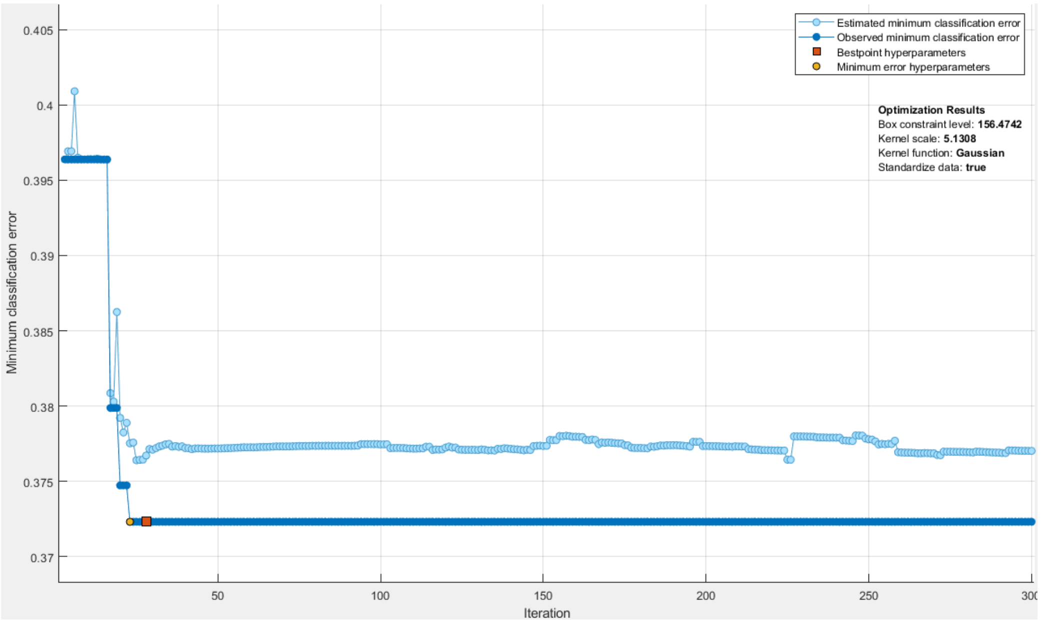


(af) SVM, XRB, LLT-based fs.

Figure S2: Confusion matrices

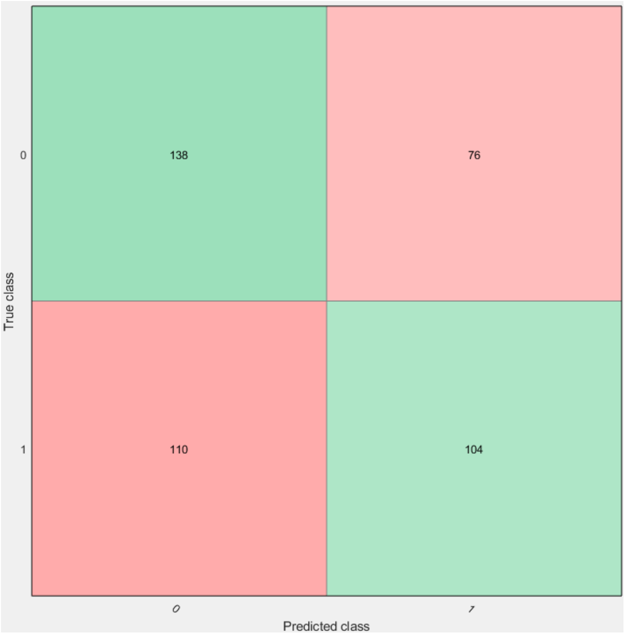


(a) Ensemble, BTC, original fs.

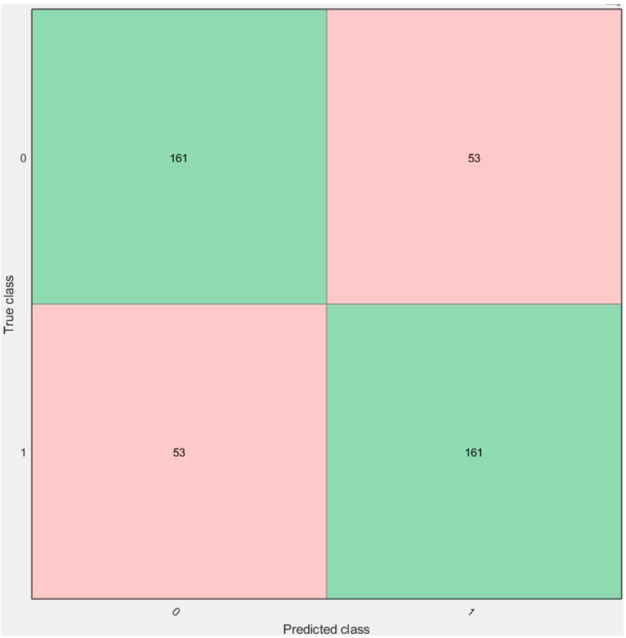


(b) Ensemble, BTC, LLT-based fs.

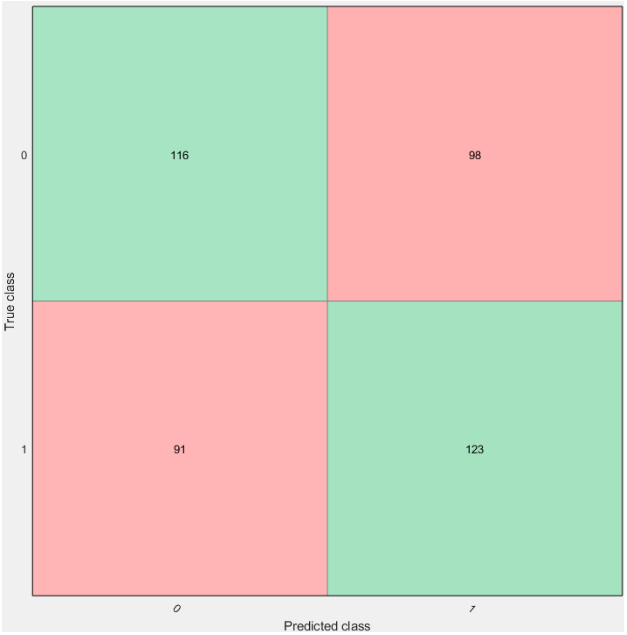


(c) Ensemble, ETH, original fs.

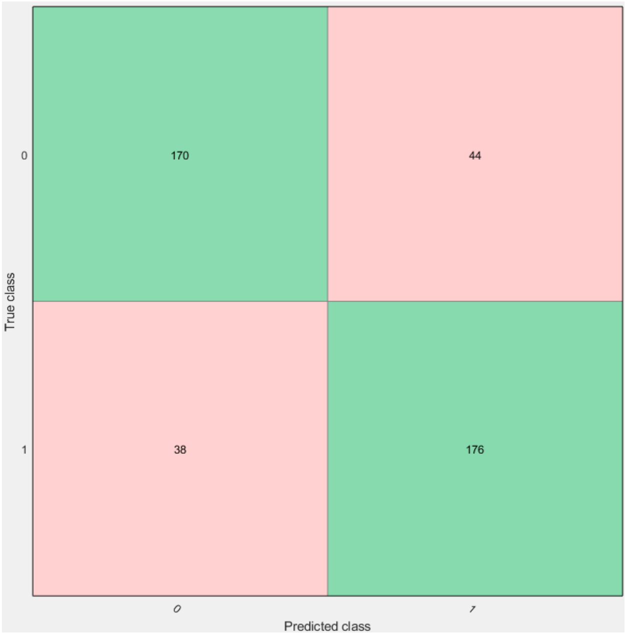


(d) Ensemble, ETH, LLT-based fs.

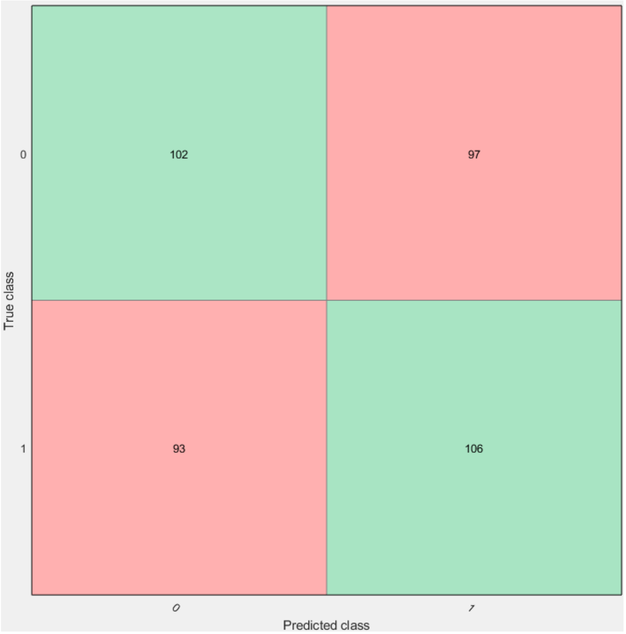


(e) Ensemble, BNB, original fs.

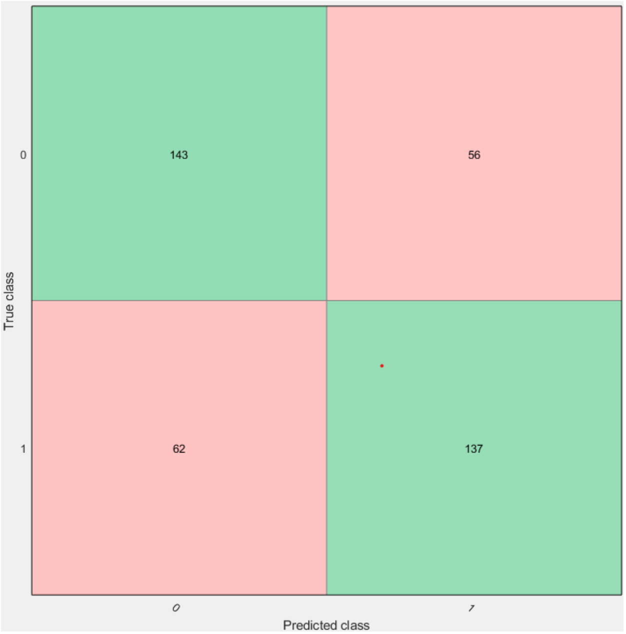


(f) Ensemble, BNB, LLT-based fs.

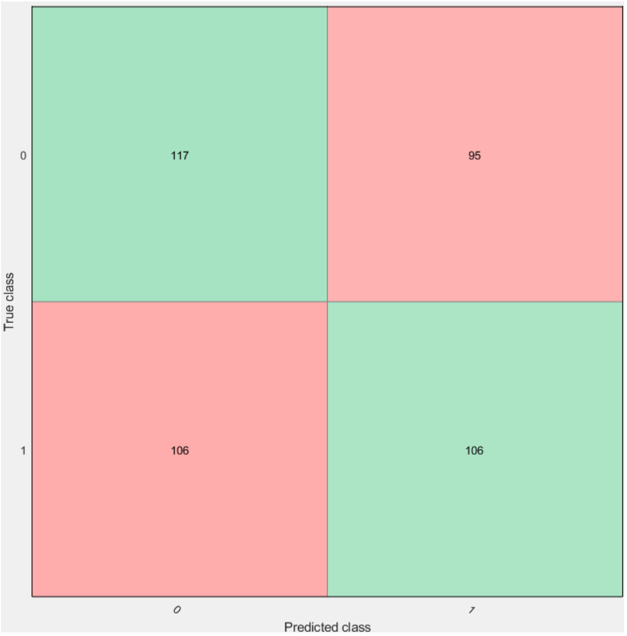


(g) Ensemble, XRB, original fs.

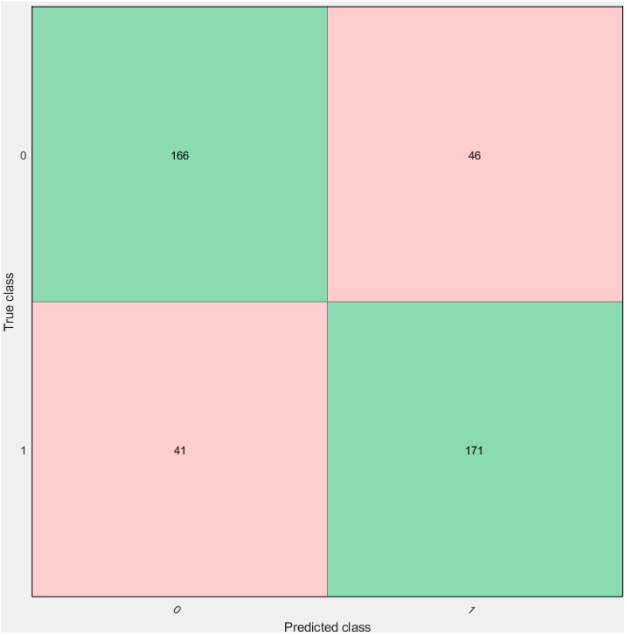


(h) Ensemble, XRB, LLT-based fs.

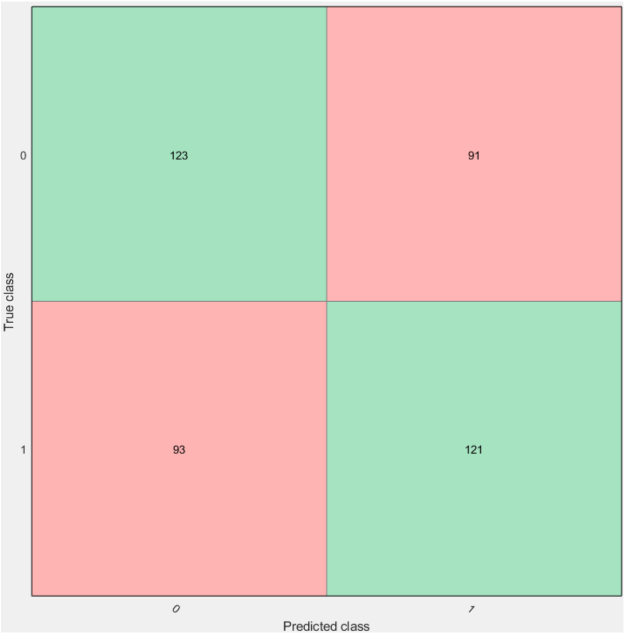


(i) KNN, BTC, original fs.

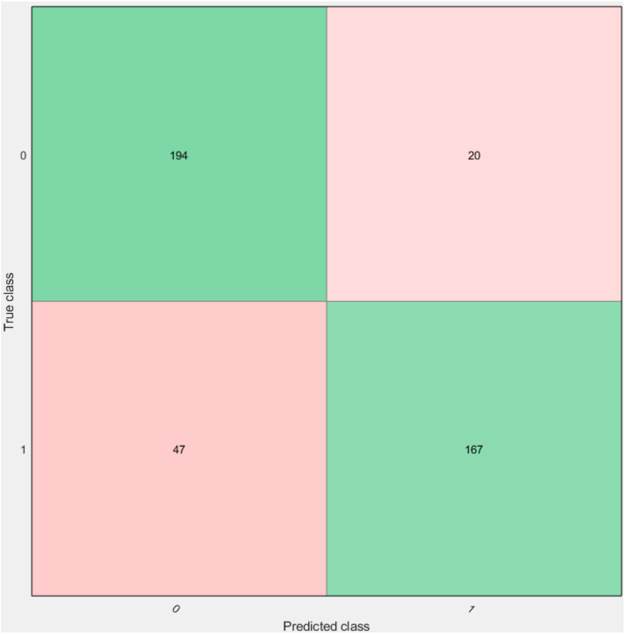


(j) KNN, BTC, LLT-based fs.

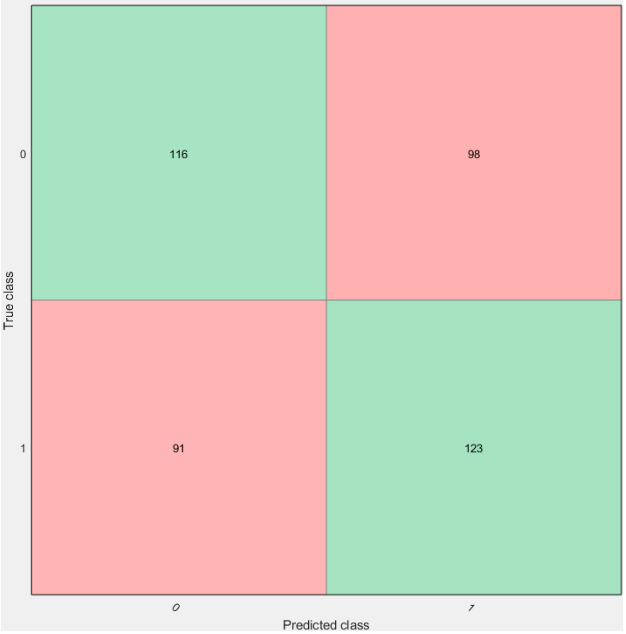


(k) KNN, ETH, original fs.

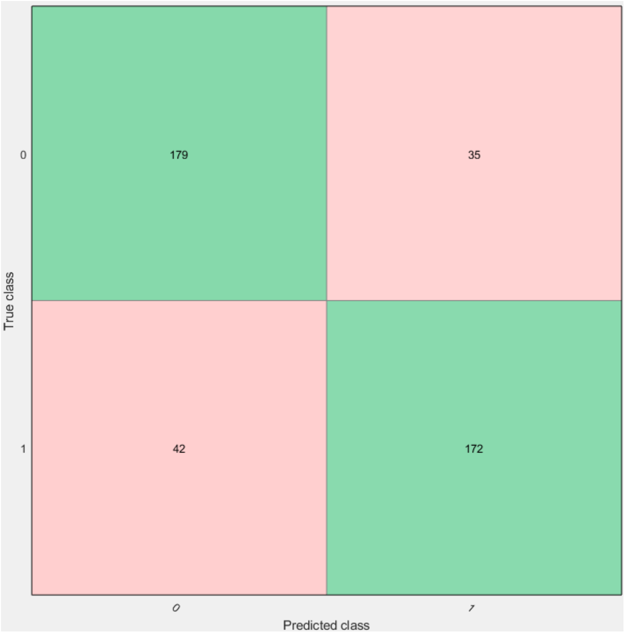


(l) KNN, ETH, LLT-based fs.

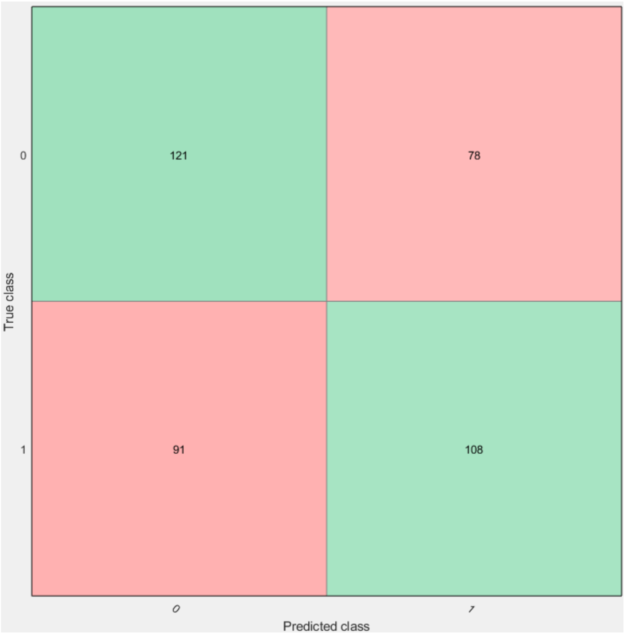


(m) KNN, BNB, original fs.

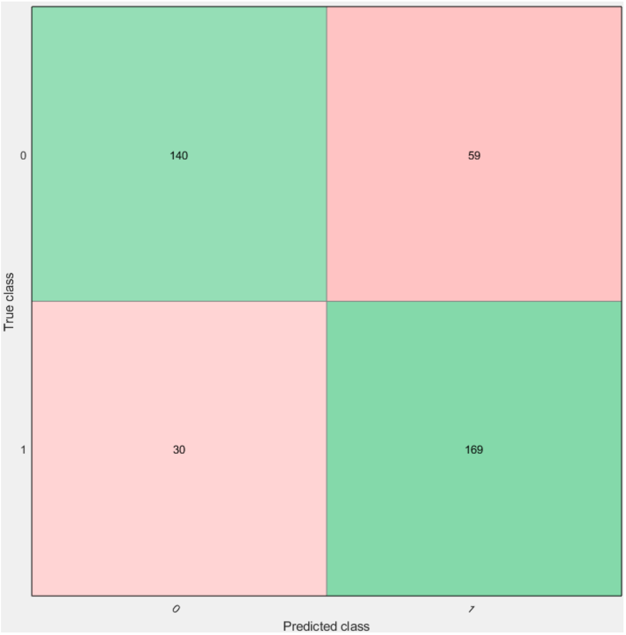


(n) KNN, BNB, LLT-based fs.

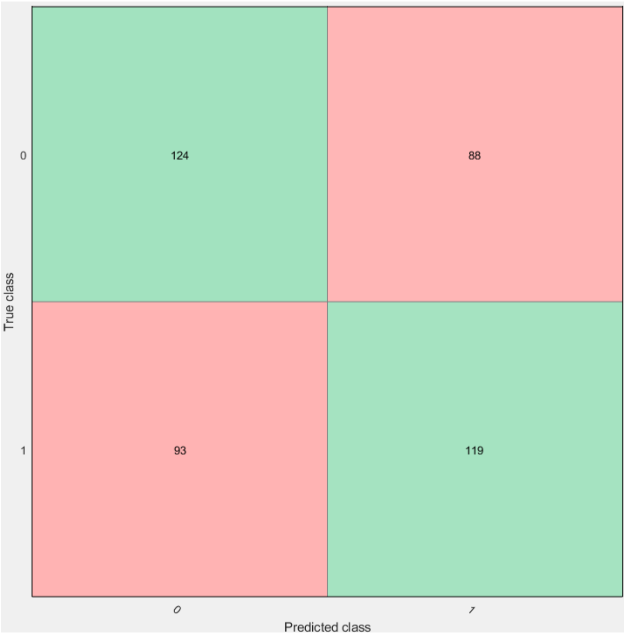


(o) KNN, XRB, original fs.

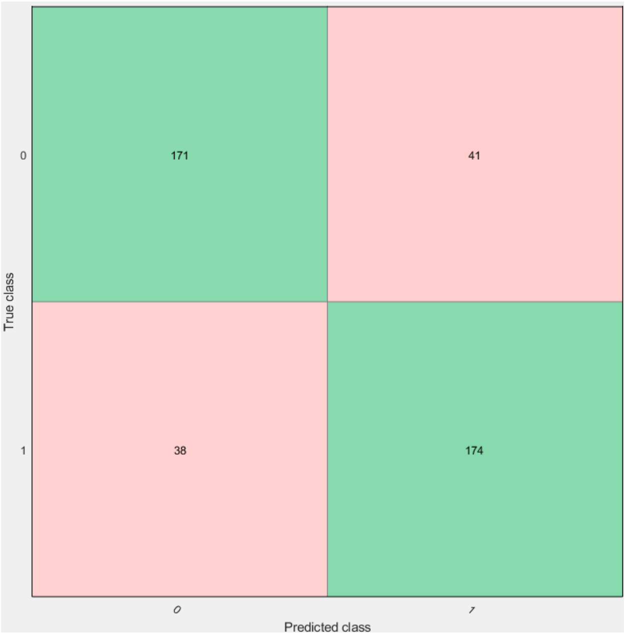


(p) KNN, XRB, LLT-based fs.

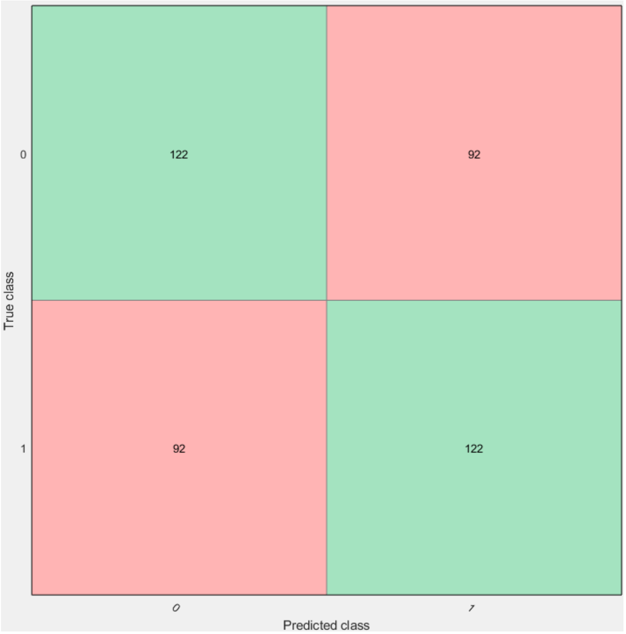

(q) DT, BTC, original fs.

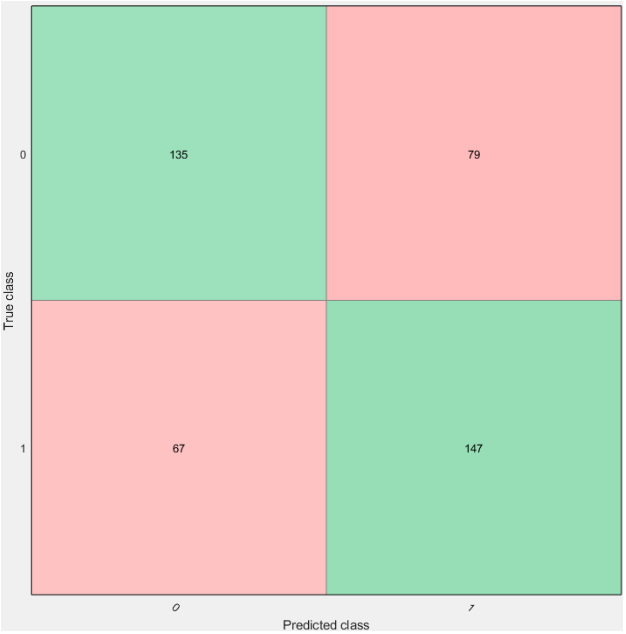

(r) DT, BTC, LLT-based fs.

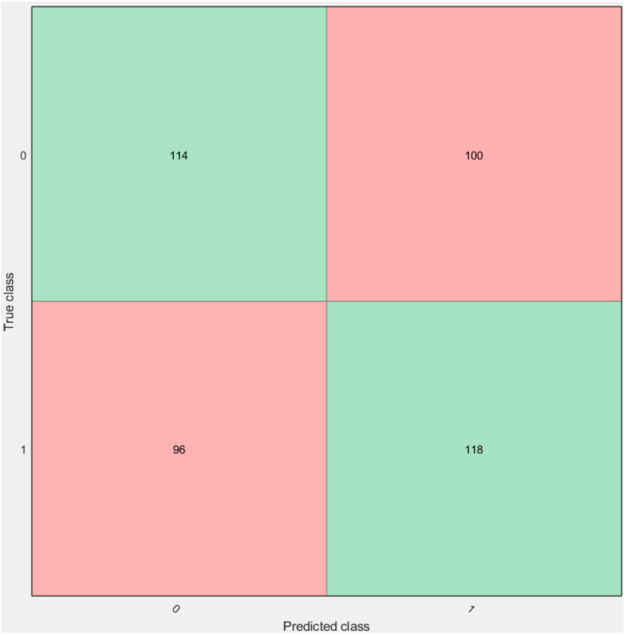


(s) DT, ETH, original fs.

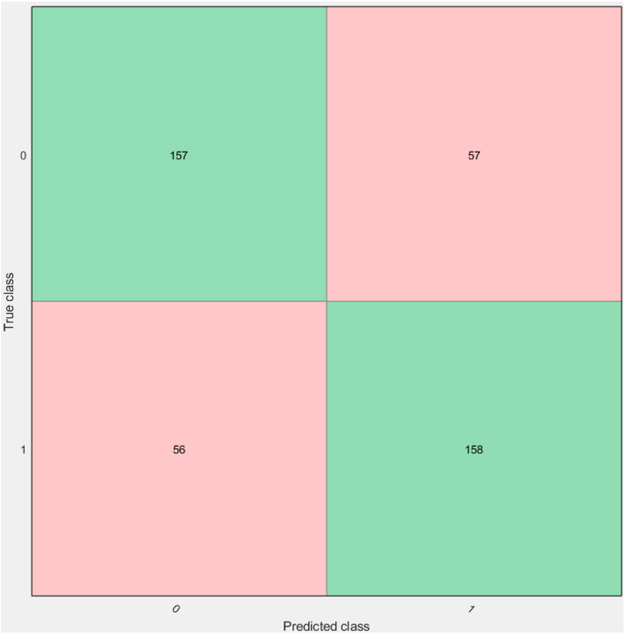


(t) DT, ETH, LLT-based fs.

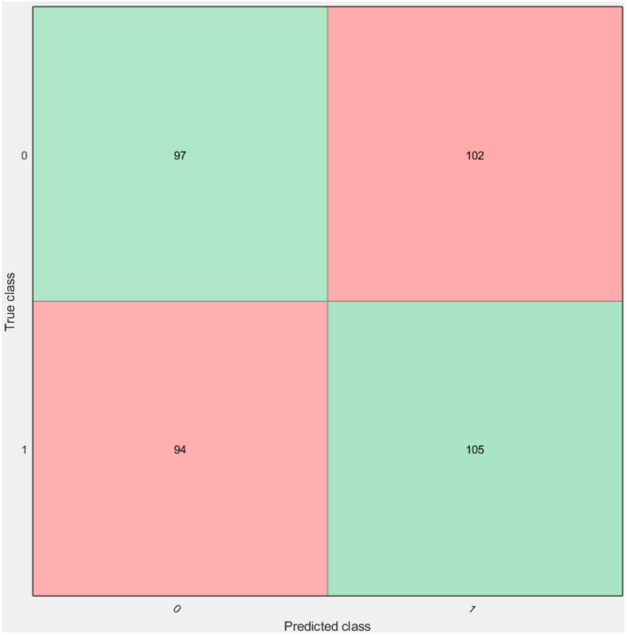


(u) DT, BNB, original fs.

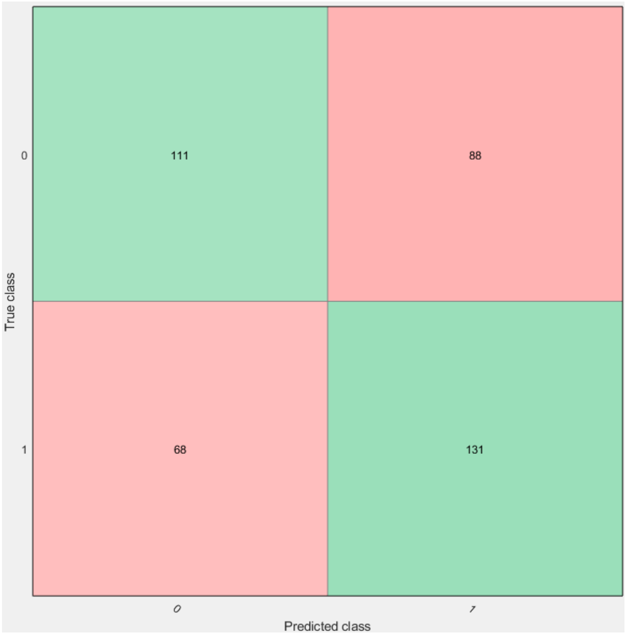


(v) DT, BNB, LLT-based fs.

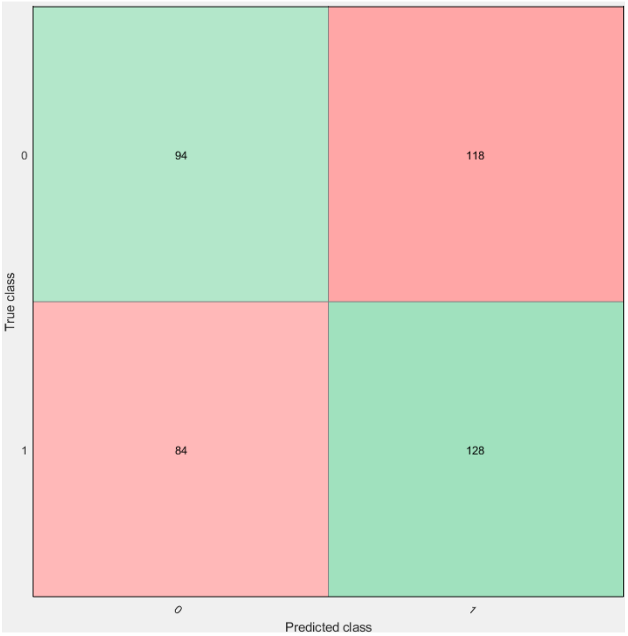


(w) DT, XRB, original fs.

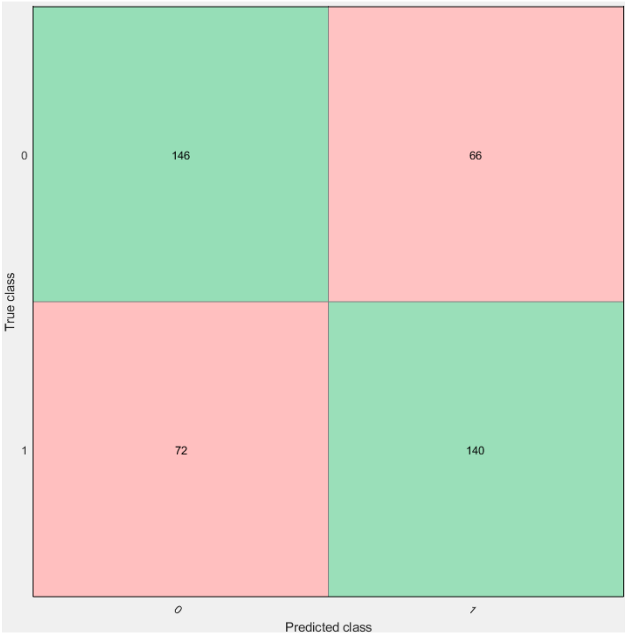


(x) DT, XRB, LLT-based fs.

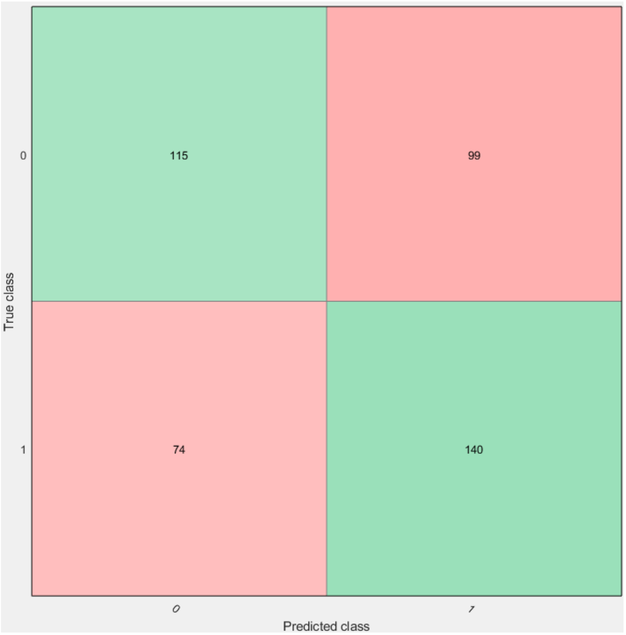

(y) SVM, BTC, original fs.

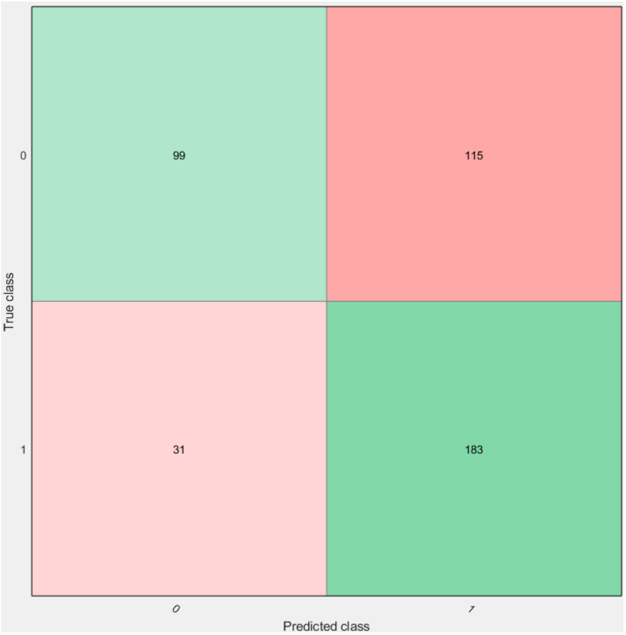

(z) SVM, BTC, LLT-based fs.

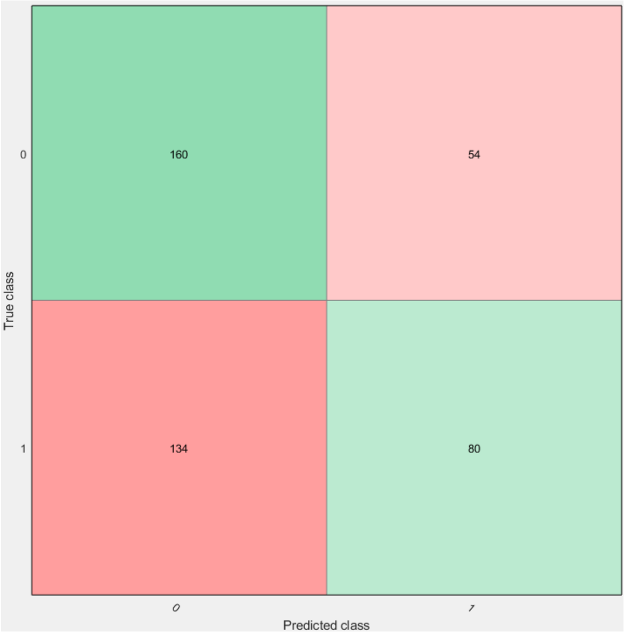


(aa) SVM, ETH, original fs.

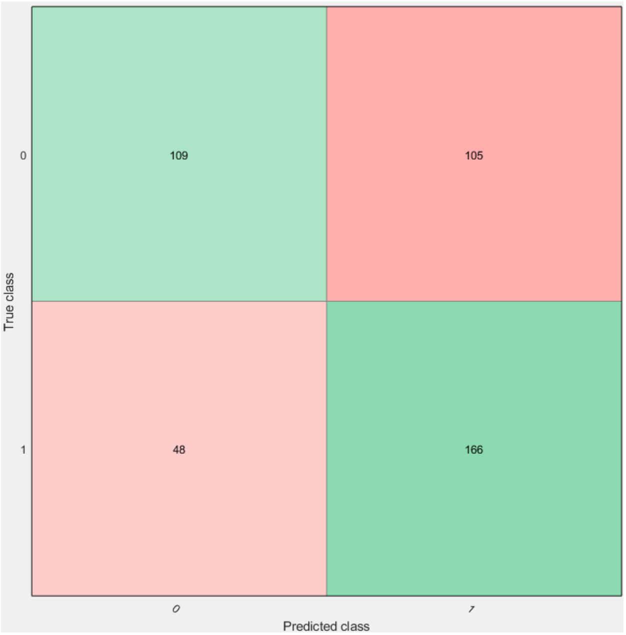


(ab) SVM, ETH, LLT-based fs.

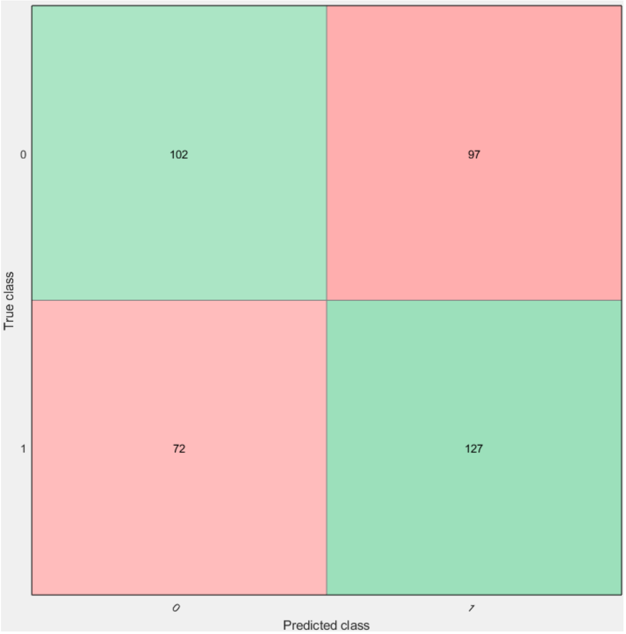

(ac) SVM, BNB, original fs.

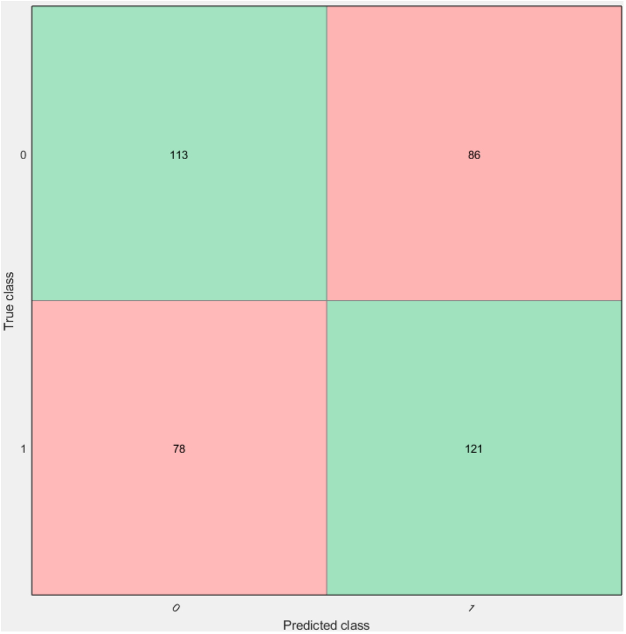

(ad) SVM, BNB, LLT-based fs.

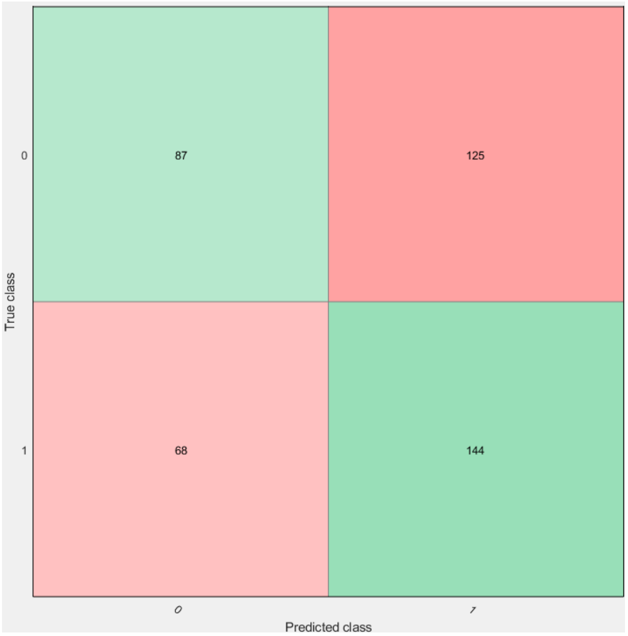


(ae) SVM, XRB, original fs.

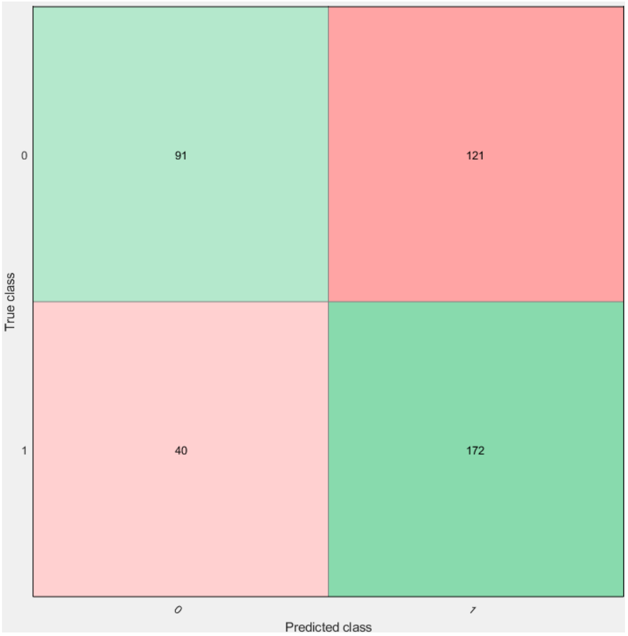


(af) SVM, XRB, LLT-based fs.
